# Supplementary material for: ECDSA.Fail: Open Autoresearch for Optimizing Elliptic-Curve Point Addition in Shor's Algorithm
Source: arXiv:2609.09582 source file (2026-09-19)
Supplement: Supplementary file 1 [file 07-appendix-results-detail.tex]

\section{Detailed Results and Circuit-Improvement Trajectory}
\label{sec:supp-results-detail}

\subsection{Overall Summary of Results}
\label{sec:supp-results-summary}


Under its official scalar objective, the challenge produced a product-score
incumbent. Viewed as a two-resource experiment, however, the public archive does
not reduce to that single point. It discloses a sparse sample of
validator-supported operating points, each instantiating a different answer to
the reversible-information question: which values must remain live, and which
may instead be recomputed, encoded, measured, or borrowed? For a submitted
circuit $c$, let $Q(c)$ denote peak logical width, $T(c)$ the average number of
executed Toffoli gates over the challenge validation support, and
$S(c)=Q(c)T(c)$ the scalar score defined in \Cref{sec:cost}. The principal
empirical result is therefore an archive-conditioned set of operating points and
transitions, not a winning number or a continuously reconstructed resource
surface.

Unless stated otherwise, quantitative archive claims in this section use the
public-ledger snapshot of 2 July 2026. A six-row source audit completed on 12
July changes the attribution of several mechanisms but not the operating points
reported here. This fixed data cutoff explains small differences from later
headline records quoted elsewhere in the evolving paper.

Within that snapshot, the first promoted baseline, submission
\texttt{30c8ded}, used $2{,}715$ peak logical qubits and $3{,}960{,}753$
average executed Toffoli gates, for a score of $10{,}753{,}444{,}395$. The best
product-score submission in the same record, \texttt{71f5115}, used $1{,}152$
qubits and $1{,}364{,}230$ average executed Toffoli gates, for a score of
$1{,}571{,}592{,}960$. Relative to the baseline, peak width fell by $57.6\%$,
average executed Toffoli by $65.6\%$, and the product objective by $85.4\%$, a
$6.84$-fold improvement. The same row is also the lowest-Toffoli promoted
circuit in this data cutoff. This conjunction records where the
product-oriented search finished; it does not imply that the two objectives are
generally aligned.

The lowest-width admitted validator-clean circuit lies on a different branch.
Submission \texttt{b6f2b0a} reached $825$ logical qubits while requiring
$489{,}161{,}900$ average executed Toffoli gates, approximately $359$ times the
count of \texttt{71f5115}. Its product score is correspondingly poor, but the
row is scientifically informative: it demonstrates a validator-clean
implementation of the point-addition primitive at a width far below the
product-score incumbent when transcript, quotient, and route information are
compressed into metadata and recomputation. The extreme-width branch thus
encounters a steep reversible time--space trade-off
\cite{bennett89,buhrman01}. Source reconstruction identifies metadata and
denominator-witness lifetime as the immediate constraints within the observed
route family.

\subsubsection{Headline operating points}
\label{sec:supp-headline-operating-points}

The benchmark evidence requires two qualifications. First,
\emph{validator-clean} means that a submission or archived public note records a
clean run over the $9{,}024$ Fiat--Shamir-derived validation instances,
including the classical, phase, and ancilla channels described in
\Cref{sec:evaluator}; it is not an all-input theorem. Second, average executed
Toffoli is the challenge metric, not necessarily a static emitted-gate count,
$T$-depth, or fault-tolerant hardware cost. The archive does not report
per-instance dispersion, so these averages are descriptive statistics over the
fixed validation support and do not imply a population confidence interval.

For the Pareto construction and related summaries, we call a row
\emph{evidence-admitted} if it is promoted or if a rejected submission has a
public note reporting a complete validator-clean $9{,}024$-instance run and
satisfies the supplementary curation rule. This conservative rule may omit
valid circuits whose validation evidence did not survive. The constructions
below are therefore conditional on the archive, not exhaustive over every
circuit that may have been produced. Hereafter, ``admitted'' has this
evidential meaning.

\begin{table}[t]
  \centering
  \small
  \setlength{\tabcolsep}{4pt}
  \begin{tabular}{@{}>{\raggedright\arraybackslash}p{3.15cm}lrrr@{}}
    \toprule
    \textbf{Operating point} & \textbf{Submission} & \textbf{$Q$} &
    \textbf{$T$} & \textbf{$QT$} \\
    \midrule
    Initial promoted baseline & \texttt{30c8ded} & $2{,}715$ & $3{,}960{,}753$ & $10{,}753{,}444{,}395$ \\
    Product-score endpoint & \texttt{71f5115} & $1{,}152$ & $1{,}364{,}230$ & $1{,}571{,}592{,}960$ \\
    Low-$Q$/score bridge & \texttt{1c0e0e9} & $1{,}133$ & $1{,}460{,}511$ & $1{,}654{,}758{,}963$ \\
    Near-$1{,}000$ clean route & \texttt{a77c9da} & $1{,}019$ & $31{,}051{,}277$ & $31{,}641{,}251{,}263$ \\
    Sub-$1{,}000$ Pareto point & \texttt{4352cfb} & $980$ & $28{,}847{,}321$ & $28{,}270{,}374{,}580$ \\
    Sub-$950$ Pareto point & \texttt{a3b0148} & $948$ & $54{,}781{,}961$ & $51{,}933{,}299{,}028$ \\
    Lowest admitted width & \texttt{b6f2b0a} & $825$ & $489{,}161{,}900$ & $403{,}558{,}567{,}500$ \\
    \bottomrule
  \end{tabular}
  \caption{Representative operating points in the 2 July data cutoff. $Q$ is
  peak logical width and $T$ is average executed Toffoli. Rejected rows are used
  only when admitted under the validation-evidence rule above.}
  \label{tab:headline-operating-points}
\end{table}

\Cref{tab:headline-operating-points} yields two immediate conclusions. The
product-score incumbent is not a proxy for minimum admitted width, and the
lowest-width admitted artifact is not product-efficient. Their separation
records how aggressively recomputation, encoded control, and reversible
witnesses can replace resident state before nonlinear work becomes prohibitive.

\subsubsection{Three empirical constructions}
\label{sec:supp-three-empirical-constructions}

The results are most legible through three related but non-equivalent
constructions. The first is a historical scalar-incumbent sequence, the second
is a mechanism-oriented low-width track, and the third is a cross-sectional
Pareto set at the data cutoff. Keeping them distinct avoids using
``frontier'' for three mathematically different objects.

The \emph{product-score incumbent sequence} comprises promoted submissions that
reduced $Q \times T$ when submitted. It culminates at \texttt{71f5115} and captures the
main trajectory of the public leaderboard. Its largest architectural movements
came from decomposing peak width into named owners, folding and hosting
inversion transcripts, compressing branch-local control, and releasing carries
or predicates at their actual final consumer. This is the construction for
which the archive supports its most complete claims about cumulative
optimization.

The \emph{validator-supported low-width track} is a mechanism-oriented
selection of admitted circuits below the product-efficient regime. It is
neither a chronological record sequence nor the set of global minimizers of
$Q$. A row enters this track because it is an admitted Pareto point, a
source-backed explanatory case, or an admitted neighbouring control used to
delimit a reported transition. In ledger order, the resulting q980, q988,
q952, q1019, q948, q828, q826, and q825 regimes replace resident arithmetic
state to varying degrees with narrower schedules, metadata, and replay. Because
this track is selected for explanatory contrast, it supports mechanism
comparison rather than frequency estimates over all low-width submissions.

The \emph{admitted $(Q,T)$ Pareto set} is the only one of these constructions
that is a frontier in the usual multi-objective sense. If $\mathcal{A}$ denotes the admitted rows, then
%
\iffalse % The formal Pareto definition is retained in the main text.
\begin{equation}
  \begin{aligned}
  \mathcal{P}(\mathcal{A})=\{c\in\mathcal{A}:{}&\nexists d\in\mathcal{A}
  \text{ such that } Q(d)\le Q(c),\ T(d)\le T(c),\\[-2pt]
  &\text{with at least one inequality strict}\}.
  \end{aligned}
  \label{eq:admitted-pareto}
\end{equation}
\fi
%
At the data cutoff this set contains seven non-dominated operating points: six
rejected low-$Q$ rows supported by full-validation notes admitted under the
curation rule, and the promoted product tip. The public branch and submission
model retained these artifacts even though a winner-only leaderboard would
have discarded them, exposing otherwise hidden trade-offs and resource
obstructions.

\iffalse % The Pareto table is retained in the main text.
\begin{table}[t]
  \centering
  \small
  \setlength{\tabcolsep}{4pt}
  \begin{tabular}{@{}lrr>{\raggedright\arraybackslash}p{5.35cm}@{}}
    \toprule
    \textbf{Submission} & \textbf{$Q$} & \textbf{$T$} & \textbf{Interpretation} \\
    \midrule
    \texttt{b6f2b0a} & $825$ & $489{,}161{,}900$ & Lowest admitted width. \\
    \texttt{f1d8707} & $826$ & $479{,}337{,}428$ & One additional qubit coincides with $9{,}824{,}472$ fewer Toffoli. \\
    \texttt{39a9b5f} & $828$ & $448{,}102{,}916$ & Two further qubits coincide with $31{,}234{,}512$ fewer Toffoli. \\
    \texttt{a3b0148} & $948$ & $54{,}781{,}961$ & Exit from the hard-$Q$ metadata cliff. \\
    \texttt{4352cfb} & $980$ & $28{,}847{,}321$ & Lowest admitted $T$ below $1{,}000$ qubits. \\
    \texttt{1c0e0e9} & $1{,}133$ & $1{,}460{,}511$ & Bridge toward the product-efficient regime. \\
    \texttt{71f5115} & $1{,}152$ & $1{,}364{,}230$ & Product-score and lowest-$T$ promoted endpoint. \\
    \bottomrule
  \end{tabular}
  \caption{The archive-conditioned Pareto set at the data cutoff. Adjacent
  differences are descriptive secants between distinct circuit families, not
  causal marginal effects.}
  \label{tab:admitted-pareto}
\end{table}
\fi

The trade-offs in \Cref{tab:admitted-pareto} are highly non-uniform. Moving from
$826$ to $828$ qubits coincides with $31{,}234{,}512$ fewer average executed
Toffoli gates, approximately $15.6$ million per added qubit. Moving from $980$
to $1{,}133$ qubits coincides with a reduction of more than $27$ million
Toffoli, whereas the final nineteen-qubit movement from $1{,}133$ to $1{,}152$
coincides with only $96{,}281$ fewer. These secant rates are not causal marginal
effects or theoretical lower bounds: the points arise from different route
families. They nevertheless provide evidence for a steep hard-$Q$ transition
among the observed routes.

\subsubsection{Fixed-budget slices}
\label{sec:supp-fixed-budget-slices}

The archive was not generated by a preregistered fixed-budget experiment:
participants optimized different objectives at different times. The following
rows are therefore ex post slices rather than controlled budget trials. For a
peak-width ceiling $q$, each row reports the admitted circuit with minimum $T$
among those satisfying $Q\le q$.

\begin{table}[t]
  \centering
  \small
  \begin{tabular}{@{}rrrrl@{}}
    \toprule
    \textbf{Budget} & \textbf{Submission} & \textbf{$Q$} & \textbf{$T$} & \textbf{Status} \\
    \midrule
    $1{,}200$ & \texttt{71f5115} & $1{,}152$ & $1{,}364{,}230$ & promoted \\
    $1{,}150$ & \texttt{1c0e0e9} & $1{,}133$ & $1{,}460{,}511$ & admitted \\
    $1{,}050$ & \texttt{4352cfb} & $980$ & $28{,}847{,}321$ & admitted \\
    $1{,}000$ & \texttt{4352cfb} & $980$ & $28{,}847{,}321$ & admitted \\
    $950$ & \texttt{a3b0148} & $948$ & $54{,}781{,}961$ & admitted \\
    $900$ & \texttt{39a9b5f} & $828$ & $448{,}102{,}916$ & admitted \\
    \bottomrule
  \end{tabular}
  \caption{Minimum admitted average executed-Toffoli cost at or below selected
  peak-qubit budgets. ``Admitted'' follows the evidence rule in the main text;
  only the scalar incumbent was promoted by the challenge.}
  \label{tab:supp-fixed-budget-slices}
\end{table}

The identical $1{,}050$- and $1{,}000$-qubit rows in
\Cref{tab:supp-fixed-budget-slices} are not a transcription error: no admitted
circuit between $981$ and $1{,}050$ qubits improves on the q980 row's executed
count. This repetition is evidence of the archive's discrete and uneven
coverage. A controlled extension would choose width ceilings in advance, fix
the validator and compute budget, and run the same agent workflow independently
at each ceiling.

\subsubsection{External results}
\label{sec:supp-external-pa-comparison}

Cross-work comparison is meaningful only when the measured object remains
visible. Babbush et al.\ report point-addition operating points in a
zero-knowledge proof package. Schrottenloher publishes explicit and tested
point-addition architectures, TrailMix supplies open implementation routes, and
{\challengename} reports public challenge submissions under its own
validator for executed cost \cite{google26,s26,trailmix}. Full ECDLP estimates,
distributed per-node estimates, and physical fault-tolerant costs are different
objects. \Cref{tab:external-pa-comparison} is therefore a map of neighbouring
operating points, not a ranking.

\iffalse % The external-comparison table is retained in the main text.
\begin{table}[t]
  \centering
  \scriptsize
  \setlength{\tabcolsep}{3pt}
  \renewcommand{\arraystretch}{1.12}
  \begin{tabular}{@{}>{\raggedright\arraybackslash}p{2.5cm}rr>{\raggedright\arraybackslash}p{5.25cm}@{}}
    \toprule
    \textbf{Artifact} & \textbf{$Q$} & \textbf{Reported count} & \textbf{Interpretation} \\
    \midrule
    Google/Babbush low-$Q$ \cite{google26} & $1{,}175$ & $2.7$M & Disclosed point-addition target; source unavailable for mechanism comparison. \\
    Google/Babbush low-gate \cite{google26} & $1{,}425$ & $2.1$M & Width/gate trade-off in the same external package. \\
    Schrottenloher space-optimized \cite{s26} & $1{,}192$ & $2^{21.19}$ & Reproducible architecture plus window cost. \\
    Schrottenloher gate-optimized \cite{s26} & $1{,}446$ & $2^{20.83}$ & Reproducible gate-oriented comparator. \\
    TrailMix \texttt{jump-lowqubit} \cite{trailmix} & $1{,}169$ & $2.09$M & Immediate open implementation prior near the low-$Q$ region. \\
    TrailMix \texttt{shrunken-PZ} \cite{trailmix} & $1{,}050$ & $32.3$M & Architectural prior for the q1019--q952 family. \\
    {\challengename} \texttt{71f5115} & $1{,}152$ & $1{,}364{,}230$ & Average executed count under the challenge validator. \\
    {\challengename} \texttt{b6f2b0a} & $825$ & $489{,}161{,}900$ & Extreme-width evidence, not an efficient full-Shor point. \\
    \bottomrule
  \end{tabular}
  \caption{Public point-addition operating points under heterogeneous accounting
  rules. ``Reported count'' is not a uniform gate metric across rows.}
  \label{tab:external-pa-comparison}
\end{table}
\fi

The headline numbers for \texttt{71f5115} are lower on both axes than those
reported for the $1{,}175$-qubit Babbush et al.\ point and the open TrailMix
\texttt{jump-lowqubit} route. This numerical ordering is not an ordering under a
common measurement model. {\challengename} counts average executed Toffoli under
its validator, some local routes exploit a classical second point, and full
window-compatible Shor usage requires the separately validated
lookup/use/unlookup construction discussed in the next subsection. The
cross-work evidence therefore places {\challengename} in the same broad
low-thousands-qubit, low-millions-Toffoli region as neighbouring public results
under its own accounting rules. Its distinctive contribution to this comparison
is traceability of source history, rejected branches, and local proof
obligations, not a cross-harness rank claim.

\subsubsection{Evidential status and selection scope}
\label{sec:supp-evidential-status}

Claims from the archive vary along two independent dimensions: correctness
evidence and benchmark-support selection. On the first dimension, an
\emph{exact local transformation} has a value-, quantum-phase-, and
ancilla-preserving argument under stated local preconditions. Controlled-swap
boundary fusion, exact chunk-boundary clearing, and a borrowed carry lane
restored to zero are examples. This supports the local mechanism claim, but it
does not prove every parameterization of the enclosing circuit. A
\emph{validator-clean circuit}, by contrast, is a complete submitted route with
$9{,}024$-instance validation recorded officially or in a public note admitted
under the curation rule. This is strong benchmark evidence but remains finite
and support-specific.

The second dimension records selection scope. A \emph{support-selected route}
may choose truncated comparison windows, width envelopes, q-cap schedules,
rerolls, or tail nonces against the benchmark support. Such a route may contain
exact local helpers and may be validator-clean as a whole; support selection
does not negate either fact. It does block an all-input exactness claim unless a
separate proof covers inputs outside the selected support. We consequently
reserve exactness claims for source-backed transformations with named local
preconditions, describe complete circuits as validator-clean under the stated
challenge procedure, and report support selection independently. Formal
circuit-family correctness and full-Shor compatibility remain additional proof
obligations.

\subsubsection{Summary interpretation}
\label{sec:supp-summary-interpretation}

The central result is not merely that $QT$ fell. The public search
repeatedly changed what counted as the scarce object. At first it was an
explicit carry or scratch register. It then became a co-owned peak, a resident
inversion transcript, a future-owned host location, a branch-window predicate,
a denominator witness, and finally a single carry whose lifetime had been
conservatively over-approximated. The low-$Q$ branch completes the picture:
when increasingly many resident values are converted into metadata or
recomputation, width continues to fall but Toffoli cost rises by orders of
magnitude. Together, the incumbent sequence, low-width track, and admitted
Pareto set provide an empirical anatomy of how reversible information was
represented and transformed within this challenge's optimization lineage for
\texttt{secp256k1} point addition.


\subsection{Detailed Circuit-Improvement Chronology}
\label{sec:supp-circuit-trajectory}

The trajectory is best read as a sequence of changing resource models. A
narrative based only on the leaderboard would present hundreds of descending
scores and suggest steady progress. The public record shows a more structured process:
long periods of nonce search and local shaving were interrupted by commits that
changed the representation of the circuit's live information. Those commits
did not merely improve the current design; by altering the location or lifetime
of the peak, they made different optimizations technically accessible and newly
valuable.

The archived dataset contains $780$ public submissions: $397$ promoted, $229$
rejected, and $154$ failed. A first-pass heuristic classifier assigns the $397$
promoted rows to $126$ nonce or micro shavings, $112$ local Toffoli
optimizations, $60$ structural optimizations, $51$ local width shavings, $28$
regime transitions, $18$ architecture or regime shifts, one structural width
cut, and one baseline. These categories are editorial rather than intrinsic
properties of the commits, and no inter-rater agreement statistic is claimed.
They characterize the curation pipeline rather than observer-invariant natural
classes. The imbalance is nevertheless informative: most promoted movement was
exploitative, whereas a much smaller set of architectural episodes changed what
subsequent search could productively optimize.

The three eras below are an ex post analytical periodization, not stages fixed
before the search. We use causal language in a process-tracing sense over
software artifacts \cite{kagdi07,hassan08}: a later optimization is described as
enabled by an earlier one only when temporal order, source changes, route notes,
and the later mechanism's preconditions form a coherent dependency chain.
Temporal succession alone is not causation. The descriptive unit is the
submission row; the unit of mechanism-level interpretation is the
\emph{mechanism episode}: an enabling source change, its proof obligations, the
operating-point movement, and nearby controls or failures that delimit the
claim. This supports a bounded dependency interpretation, not experimental
identification of the episode's isolated effect.

\subsubsection{Optimization of the logical width--work product}
\label{sec:supp-product-trajectory}


\iffalse % The trajectory figure and reviewer note are retained in the main text.
\begin{figure}[p]
  \centering
  \captionsetup[sub]{font=small,labelfont=bf,justification=justified,%
    singlelinecheck=false}

  \begin{subfigure}{\linewidth}
    \centering
    \resizebox{0.82\linewidth}{!}{\input{figs/qxt-error-dual-axis-plot}}
    \caption{Point-addition circuit score. The left axis compares the standard
    $Q\times T$ score with the correctness-adjusted $Q\times T/p$ score. The faded
    right-axis curve reports the measured error rate $100(1-p)$.}
    \label{fig:qxt-shor-comparison-pa}
  \end{subfigure}

  \vspace{0.35cm}

  \begin{subfigure}{\linewidth}
    \centering
    \resizebox{0.82\linewidth}{!}{\input{figs/shor-circuit-estimate-plot}}
    \caption{Estimated full Shor circuit cost. The raw estimate is
    $28\times Q'\times T'$, while the correctness-adjusted estimate is
    $28\times Q'\times T'/(1-28e)$. The faded right-axis curve shows the amplified
    error $28e$, and the three local score reversals are highlighted.}
    \label{fig:qxt-shor-comparison-full}
  \end{subfigure}

  \caption{Resource-cost evolution across the sampled accepted submissions. Both
  panels use the same random set of $50{,}000$ elliptic-curve point pairs per
  commit. Following the windowed full-attack estimate~\eqref{eq:full-attack}, the
  full-circuit panel uses $Q'=Q+16$, $T'=T+3\cdot2^{16}$, and $e=1-p$, with
  $2n/w-4=28$ point additions at $n=256$ and $w=16$ (\Cref{sec:ecc-quantum}). The
  right axes report error-related quantities.}
  \label{fig:qxt-shor-comparison}
\end{figure}

% \begin{figure}[tp]
%   \centering
%   \resizebox{\linewidth}{!}{\input{figs/qxt-error-dual-axis-plot}}\\[2pt]
%   {\small\textbf{(b) Point-addition circuit score.} The left axis compares the
%   standard $Q\times T$ score with the correctness-adjusted $Q\times T/p$
%   score. The faded right-axis curve reports the measured error rate
%   $100(1-p)$.}

%   \vspace{0.35cm}

%   \resizebox{\linewidth}{!}{\input{figs/shor-circuit-estimate-plot}}\\[2pt]
%   {\small\textbf{(a) Estimated full Shor circuit cost.} The raw estimate is
%   $28\times Q'\times T'$, while the correctness-adjusted estimate is $28\times Q'\times T'/p'$ where $p' = (1-28e)$. The faded
%   right-axis curve shows the amplified error $28e$, and the three local score reversals are highlighted.}

%   \caption{Resource-cost evolution across the sampled accepted submissions. Both
%   panels use the same fixed set of $50{,}000$ elliptic-curve point pairs per
%   commit. Following the windowed full-attack estimate~\eqref{eq:full-attack}, the
%   full-circuit panel uses $Q'=Q+16$, $T'=T+3\cdot2^{16}$, and $e=1-p$, with
%   $2n/w-4=28$ point additions at $n=256$ and $w=16$ (\Cref{sec:ecc-quantum}). The right axes report error-related quantities.
%   }
%   \label{fig:qxt-shor-comparison}
% \end{figure}
\fi

The union-bound interpretation of the longitudinal proxy requires an explicit
scope condition. If $e$ were the applicable per-addition error probability, the
union bound would give $1-28e$ as a lower bound on success. The plotted
$\hat p'_{\mathrm{LB}}$ instead substitutes the empirical
$1-\hat p$ for $e$: it is a descriptive plug-in proxy, not a confidence bound,
and $\hat p$ measures classical-output agreement rather than coherent circuit
success. Only under an independently rerunnable success model would a $5\%$
composed error imply the repetition factor
$1/(1-0.05)\simeq1.053$, or approximately $5.3\%$ additional expected work.


Throughout this subsection, $QT$ denotes the challenge's product of logical
width and nonlinear work. Although sometimes called a spacetime surrogate, it
is not circuit depth, active volume, or fault-tolerant spacetime.

\paragraph{From monolithic arithmetic to jointly owned peaks.}
The baseline exposed the familiar costs of reversible modular arithmetic:
carry lanes, reduction scratch, controlled swaps, and Euclidean inversion
history \cite{cuccaro04,proos-zalka03}. Early optimization treated these as
independent targets, a view that failed whenever several phases tied for the
global maximum. Reducing one owner simply revealed another at the same height.

The \texttt{d35d6e7} episode fused consecutive Kaliski $(r,s)$ controlled swaps
across an iteration boundary (\Cref{sec:fam-fusion}). Its immediate width effect
was modest, but it established that a control value need not be materialized
twice when its forward and reverse lifetimes can be joined exactly.

The first large width movement, \texttt{f94f726}, reduced the peak to $2{,}310$
qubits. Late-iteration clean carries, future-pool borrowing, low-scratch Solinas
reduction, affine multiplication narrowing, and controlled-swap framing had to
move together. The source-backed lesson is that the global peak is a property
of overlapping owner intervals, not of the largest helper in isolation.

Once this transition exposed a stable $2{,}310$-qubit regime, the earlier
fusion idea could be extended. \texttt{112d5a4} applied the same merge to the
$(u,v_w)$ channel over its provably safe iteration prefix, reducing average
executed Toffoli to $3{,}361{,}759$ without changing the peak. Subsequent fixed-width
exploitation lowered the count to $2{,}462{,}914$ at \texttt{375fdff}. The
sequence matters: a boundary-fusion experiment preceded the broad width
transition; that transition then created a stable regime in which stronger
fusion and local optimization became valuable. Era I reduced the score from
$10.75$ billion to $5.69$ billion, but left a question that local arithmetic
tuning could not answer: why was so much inversion history still resident at
the peak?

\paragraph{From resident history to phase-local transcript.}
Here ``phase-local'' denotes a scheduled arithmetic phase; quantum phase and
phase-correction obligations are named separately where they arise.
Submission \texttt{0620443} exploited the changing shape of the Euclidean walk.
Dialog-history entries were folded into idle high bits of shrinking registers,
carry pools were relocated onto clean suffixes, and an affine square was
recomputed instead of carried. Width fell from $2{,}309$ to $2{,}025$ qubits
even as Toffoli rose slightly. Bennett-style recomputation and Luo-style
register sharing supplied the conceptual vocabulary
\cite{bennett73,bennett89,luo26}; the local contribution was an ownership map
precise enough to survive reverse replay.

That ownership map enabled \texttt{0c1d4d9} to absorb a compressed-sidecar
architecture and reduce the circuit to $1{,}698$ qubits. This was not the
invention of transcript compression or of the imported point-addition family.
Its contribution was integration: compressed-block primitives, lifecycle
replay, terminal-state handling, route defaults, and point-addition wiring were
made mutually valid under the challenge. Once explicit history ceased to be
the dominant object, the $1{,}698$-qubit band could be mined for Toffoli
reductions, falling from $2{,}447{,}846$ to $1{,}704{,}086$ average executed
Toffoli before width moved again.

Submission \texttt{744b274} converted the future transcript from passive
storage into a host. Future-owned slots carried gated registers before their
eventual owner became live, while windowed apply carries prevented the
arithmetic from recreating the peak. This reduced width to $1{,}572$ qubits and
changed the design question: after broad transcript compression, how little
branch and window information did the current arithmetic phase require?

Source inspection reconstructed six transitions whose attribution was initially
open, sharpening the cumulative sequence. In \texttt{3bd3aa5}, the circuit
materialized $f=\mathit{ctrl}\wedge a$ one chunk at a time, cleared each slice
with the benchmark's HMR X-basis demolition measurement, and removed retained
boundaries with exact controlled comparators. The resulting row used $1{,}567$
qubits and $1{,}689{,}505$ average executed Toffoli. Submission
\texttt{da05eeb} then relieved six co-binders together: it hosted the $z_0$
square carry lane, selected a low-$Q$ $z_2$ square, vented Solinas corrections,
and widened the exact apply cut, producing a $42$-qubit reduction and a
$1{,}500$-qubit operating point. With that peak displaced, \texttt{f2cd713}
hosted a fused branch comparator's carry lane on a clean future-log slice and
sank the apply phase to the next body floor, reaching $1{,}466$ qubits.

Submission \texttt{ca1cd1f} next applied phase-local reasoning to the transcript
through a high-$u$ compressed-log runway and $K=2$ bounded-shift storage. The
circuit remembered only the branch/window information needed to reverse the
current arithmetic phase, reaching $1{,}394$ qubits. The final reconstructed
transition, \texttt{67be862}, combined a low-$Q$ final ripple, a hosted
split-boundary comparator, and five balanced chunks to reach $1{,}320$ qubits.
These reconstructed rows do not each become an independent discovery. Rather,
they show that the earlier ``source gap'' label denoted an incomplete causal
evidence chain, not an inexplicable commit.

Submission \texttt{4b7d727} then exploited a different distinction: emitted
work and executed work are not the same benchmark object. Conditional replay
reduced average executed Toffoli to $1{,}404{,}058$ at $1{,}300$ qubits by
performing nonlinear work only on branches that required it. This is a
source-backed challenge-score mechanism, but not automatically a static gate
deletion or physical-resource reduction. By the end of Era II the score had
fallen to $1.83$ billion. The broad architectural objects had been compressed;
what remained were increasingly small, proof-sensitive lifetimes.

\paragraph{From broad compression to last-consumer proofs.}
The descent through the $1{,}226$--$1{,}168$-qubit region was jagged. Route
defaults, window widths, support assumptions, rerolls, and unrelated co-binders
could decide whether a one-qubit change appeared at the measured peak. Many
rows in this band remain evidence-curation targets, so their mechanisms are
left unattributed rather than reconstructed by inference. Collectively, they
show that the circuit had become a packing problem over branch-local transcript
state, shrunken arithmetic, and narrow validation islands.

The $1{,}165$--$1{,}169$ regime persisted for approximately $90.7$ hours and
$113$ public submissions before \texttt{44d7d51} entered the
$1{,}160$--$1{,}164$ bucket. The unblock was a one-bit lifecycle argument. A bit
known to be zero or one at a particular phase could host temporary information
provided its original owner was dormant and the bit was restored before that
owner returned. The general idea is old; the local scientific work was to name
the exact value, owner interval, and restoration point at a hard-pinned peak.

Submission \texttt{6c1a65d} generalized this reasoning from a bit to a schedule.
Per-call reserve maps replaced route-global scratch assumptions, final carries
were consumed directly where legal, and measured cleanup was paired with the
nonlinear phase feedback required by the branch relation
\cite{jones13,gidney18}. Finally, \texttt{71f5115} released the \texttt{cy0}
carry in the internally named FFG arithmetic schedule on suffix calls where its
last consumer could be named, while coordinated square-vent,
coordinate-truncation, reverse-subtract, and tail-swap changes prevented
adjacent phases from reclaiming the maximum.

The late product-score sequence therefore closes with a precise proposition
rather than a grand identity: this carry is dead, on these calls, after this
consumer, under this route. Progress came from replacing conservative residency
with increasingly exact statements about who owns information and when.

\iffalse % The era summary table is retained in the main text.
\begin{table}[t]
  \centering
  \small
  \setlength{\tabcolsep}{4pt}
  \begin{tabular}{@{}llrrr>{\raggedright\arraybackslash}p{3.9cm}@{}}
    \toprule
    \textbf{Stage} & \textbf{Endpoint} & \textbf{$Q$} & \textbf{$T$} & \textbf{$QT$} & \textbf{Resource model learned} \\
    \midrule
    Baseline & \texttt{30c8ded} & $2{,}715$ & $3{,}960{,}753$ & $10.75$B & Resident arithmetic modules. \\
    Era I & \texttt{375fdff} & $2{,}309$ & $2{,}462{,}914$ & $5.69$B & Peaks have overlapping owners. \\
    Era II & \texttt{4b7d727} & $1{,}300$ & $1{,}404{,}058$ & $1.83$B & History and control can be hosted and decoded locally. \\
    Era III & \texttt{71f5115} & $1{,}152$ & $1{,}364{,}230$ & $1.57$B & Late progress requires last-consumer and cleanup proofs. \\
    \bottomrule
  \end{tabular}
  \caption{Representative endpoints of the product-score trajectory. The eras
  are an ex post process-tracing periodization.}
  \label{tab:trajectory-eras}
\end{table}
\fi

\subsubsection{Low-qubit track}
\label{sec:supp-low-qubit-track}

The low-qubit track asks how far width can be reduced when Toffoli cost is not
the primary objective. Reversible computation permits time to be exchanged for
space, but the exchange rate is architecture-specific
\cite{bennett89,buhrman01}. The public rejected branches make that exchange
empirically visible for the route families under study.

TrailMix supplied the principal inbound implementation substrate. Its open
\texttt{shrunken-PZ} route reported approximately $1{,}050$ qubits and $32.3$
million Toffoli, demonstrating a qualitatively different point-addition
architecture below the main low-thousand-qubit routes \cite{trailmix}.
{\challengename} did not invent that architecture; it provided a public
environment in which the route could be ported, specialized, stress-tested,
and compared with neighbouring circuits under a common validator.

\paragraph{Sub-$1{,}000$ specialization and coordinate liveness.}
\label{sec:supp-sub1000-shrunken-pz}
Submission \texttt{cb40049}, source
\commitref{86c8e1e}{86c8e1efec09ed1a97568edfa2069fe76b129be5}, combined three
changes: a deterministically trained thin schedule followed by a
$500{,}000$-sample repair pass, an $8$-qubit completion counter, and direct
classical-register modular additions and subtractions that avoided a
$257$-qubit loaded-coordinate register in the highest-pressure coordinate
phases. The profile retained the baseline leading-zero scan and $6$-bit
shift-distance control, and selected tail nonce $2$. Its attached public note
records a clean local $9{,}024$-instance run at $Q=999$ and
$T=57{,}041{,}103$. The service row is failed and has no API metrics, so these
figures are local-note evidence rather than service-reported resource metrics.

Submission \texttt{85d5dae}, source
\commitref{f46a8c4}{f46a8c47d39bb6446beec23614799784506a984b}, then introduced
an $80$-bit leading-zero scan window, capped the quotient at $20$ qubits, and
reduced the shift-distance register to $5$ qubits while retaining the $8$-bit
counter. The source regenerated the thin schedule with seed $278$ and selected
tail nonce $602$. Its API row reports $(Q,T)=(980,39{,}648{,}420)$, and its
public note records a clean local $9{,}024$-instance run. These settings form a
joint profile: the observed reduction is not attributable to any one bound or
nonce in isolation.

The lower-work branch changed the lifetime of the forward numerator. Source
\commitref{6020c67}{6020c67a36798754f4d5253e4b9e9d52595583b1} reversed
$\Delta y=\lambda\Delta x$ immediately after the final consumer of $\Delta y$,
reused the resulting clean register for loaded-coordinate arithmetic, and
rematerialized $\Delta y'=\lambda\Delta x'$ before output-side slope
cancellation. Combined with a $78$-bit leading-zero window, step-specific shift
bounds with a one-bit safety margin, and tail nonce $3116$, this route yielded
submission \texttt{e0281a8} at $(Q,T)=(988,29{,}210{,}249)$. Submission
\texttt{4352cfb}, source
\commitref{32bd568}{32bd56898f9d5494a4922642711395e47c910f2d}, combined the
same zero-$\Delta y$ route and $78$-bit window with the $20$-qubit quotient cap,
$5$-qubit shift-distance register, deferred $y$-materialization, and tail nonce
$25$, yielding $(980,28{,}847{,}321)$. Its average executed Toffoli count is
$27.2\%$ below that of the earlier $Q=980$ profile, but this remains a
profile-level comparison because several settings changed together. The API
reports both operating points, and their attached public notes record clean
$9{,}024$-instance runs.

The subsequent chronology remained jagged. On 19 June, \texttt{0ce9b13} moved
to $952$ qubits while raising the executed count to $78{,}159{,}965$.

Later that day, the search returned to a wider $1{,}019$-qubit construction.
Submission \texttt{a77c9da} combined support scheduling, leading-zero windows,
margin and shift controls, route defaults, and diagnostic high-bit checks in a
validator-clean circuit at $31{,}051{,}277$ average executed Toffoli. Its
importance is explanatory rather than Pareto-optimal: the source record exposed
the central obstruction. A second \texttt{shrunken-PZ} cancellation suggested
an algebraic batch relation of the kind used to amortize simultaneous
inversions \cite{montgomery87,harris08}, but a reversible implementation still
needed the denominator, cofactor, inverse, and cleanup witness to have a
peak-safe owner. Carrying a full-width passenger through inversion erased the
width saving. Algebraic feasibility therefore failed to imply circuit
feasibility.

On 21 June, \texttt{a3b0148} reached $948$ qubits at $54{,}781{,}961$ Toffoli,
improving both coordinates relative to q952 but not restoring the low executed
cost of q980. The sequence is non-monotonic in both resources because support
schedules, arithmetic helpers, and metadata representations change discretely;
not every integer width has a comparably efficient circuit.

The hard-$Q$ continuation made metadata the dominant resource. Quotient
lengths, implicit high bits, route classes, hosted predicates, and reversal
witnesses were encoded instead of storing the full values they described.
Submission \texttt{39a9b5f} reached $828$ qubits at $448{,}102{,}916$ average
executed Toffoli; \texttt{f1d8707} reached $826$ at $479{,}337{,}428$; and
\texttt{b6f2b0a} reached $825$ at $489{,}161{,}900$. The final few qubits thus
cost tens of millions of additional Toffoli. Together, these points delimit the
observed hard-$Q$ cliff.

This track makes two contributions. Technically, it identifies
denominator-witness and metadata lifetime as limiting objects within the
observed routes after ordinary arithmetic scratch has been compressed.
Methodologically, it shows why rejected submissions belong in the research
record: none improved the product score, but together they reveal a resource
trade-off that the product leaderboard cannot express.

\subsubsection{Pareto-frontier exploration}
\label{sec:supp-pareto-exploration}

The Pareto status is a cross-sectional property of
the admitted set at the data cutoff. Historical promotion asks a different
question: did a row improve the scalar score when submitted? The two
classifications can disagree, particularly on a discrete, non-convex frontier
where scalarization conceals useful operating points. Only one of the seven
admitted Pareto points is the promoted product tip. The other six are rejected
low-$Q$ rows supported by full-validation notes admitted under the curation
rule.

The discreteness of the mechanisms explains why both the Pareto set and the
chronological search path are jagged. A new host becomes available only after
its future owner is proved inactive; a carry disappears only after its final
consumer is moved; a transcript shrinks only after a replay relation changes;
and a denominator batch helps only if its witness can cross the inversion peak
cheaply. These transformations create islands and cliffs rather than a smooth
family indexed by qubit count.

This observation makes the open-autoresearch argument empirically specific. A
greedy scalar leaderboard supplies exploitation pressure but can suppress
branches that spend one resource to explore another
\cite{march91,terwiesch-xu08}. The public submission ledger partially mitigated
that loss by preserving rejected commits and notes. A future challenge could
make the repair explicit by promoting the $(Q,T)$ Pareto set, maintaining
objective-specific leaderboards, or rewarding source-backed regime transitions
that do not improve the current scalar tip. Such a design would reward
validated information about the geometry of the search space, not arbitrary
regressions.


\subsubsection{Live-information model}
\label{sec:trajectory-information-model}

The mechanism episodes can be compared through the explanatory tuple
%
\begin{equation}
  \mathcal{I}=(\mathsf{value},\mathsf{width},\mathsf{location},
  \mathsf{owner},\mathsf{live\ interval},\mathsf{provenance},
  \mathsf{cleanup},\mathsf{proof\ duty}).
  \label{eq:live-information}
\end{equation}
%
This is a coding schema distilled from the source record, not a circuit theorem
or a claim of priority over reversible pebbling, register sharing, or
measurement-based uncomputation
\cite{bennett73,bennett89,kralovic04,cuccaro04,luo26,jones13,gidney18}.
It makes explicit two conditions that scalar deltas conceal: a local
transformation changes $Q$ only if its live interval intersects a measured
maximum and every phase tied at that maximum is also relieved; holding the
validation support fixed, it changes average $T$ only if it reduces executed
Toffoli work on that support. Transcript compression changes width and
provenance; hosting changes location and temporary custody; loans shorten live
intervals; measurement changes cleanup and its phase obligation; and hard-$Q$
metadata replaces a full value with a narrower description whose reversal is
more expensive. Complete field definitions and evidence requirements appear in
\Cref{tab:supp-live-information-schema}.

The trajectory is therefore an interacting sequence rather than a collection
of independent tricks. Joint-peak analysis made transcript residency visible;
compression made branch-local provenance salient; measured cleanup made phase
part of the resource contract; and low-width exploration made witness lifetime
salient. The schema organizes both the $6.84$ score ratio and the
orders-of-magnitude work increase on the extreme-width branch, but neither
decomposes those outcomes causally nor claims predictive completeness. The next
subsection changes the analytical axis from chronology to transformation
family.

\subsubsection{What the trajectory shows}
\label{sec:supp-trajectory-information-model}

Across all three tracks, the underlying research object is live information.
As an analytical abstraction distilled from the source-backed episodes above,
a local live object may be represented by the tuple in
\Cref{eq:live-information}.
%
\iffalse % The compact coding tuple is retained in the main text.
\begin{equation}
  \mathcal{I}=(\mathsf{value},\mathsf{width},\mathsf{location},
  \mathsf{owner},\mathsf{live\ interval},\mathsf{provenance},
  \mathsf{cleanup},\mathsf{proof\ duty}).
  \label{eq:live-information}
\end{equation}
\fi
%
This tuple is an explanatory coding schema, not a circuit theorem or a
canonical representation.

Its ingredients are individually established. Reversible simulation and
pebbling supply store--recompute trade-offs; reversible addition and register
sharing supply carry-lifetime and ownership patterns; and measurement-based
uncomputation supplies a distinct cleanup relation
\cite{bennett73,bennett89,kralovic04,cuccaro04,luo26,jones13,gidney18}. The
contribution claimed here is neither a new reversible-computation theorem nor
priority over those techniques. It is their empirical synthesis into a
source-auditable scheme that binds each resource transformation to a live
object, cleanup route, and proof duty, permitting comparison across
heterogeneous commits.

\begin{table}[t]
  \centering
  \scriptsize
  \setlength{\tabcolsep}{3pt}
  \renewcommand{\arraystretch}{1.12}
  \begin{tabular}{@{}>{\raggedright\arraybackslash}p{1.5cm}>{\raggedright\arraybackslash}p{3.9cm}>{\raggedright\arraybackslash}p{5.0cm}@{}}
    \toprule
    \textbf{Field} & \textbf{Meaning} & \textbf{Evidence required} \\
    \midrule
    Value & Logical datum at the relevant program point. & Forward semantics and applicable range or branch condition. \\
    Width & Logical qubits occupied at the measured peak. & Allocation or peak trace tied to the active route. \\
    Location & Physical register or slice carrying the datum. & Allocation trace and any host or alias relation at the relevant phase. \\
    Owner & Logical object whose future correctness constrains reuse. & Non-interference during borrowing and restoration before ownership returns. \\
    Live interval & Production or loan entry through final consumption or restoration. & Producer, last consumer, and reverse-path evidence. \\
    Provenance & Stored, recomputed, metadata-decoded, measured, or borrowed. & Source path establishing the current representation. \\
    Cleanup & Reversal, consumption, measurement with feedback, or exact overwrite. & Value, ancilla, and phase restoration under stated preconditions. \\
    Proof duty & Condition licensing the transformation. & Local proof, exhaustive helper test, or bounded validator evidence. \\
    \bottomrule
  \end{tabular}
  \caption{The live-information coding schema used to compare source-backed
  mechanism episodes.}
  \label{tab:supp-live-information-schema}
\end{table}

The schema describes local objects, whereas $Q$ and $T$ are global circuit
measurements. The connection is conditional. A local width reduction changes
$Q$ only when its live interval intersects a measured maximum and every phase
tied at that maximum is also relieved. Holding the validation support fixed, a
local work reduction changes $T$ only when it reduces executed Toffoli work on
that support. An exact local transformation can therefore be a genuine
mechanism without moving either headline metric by itself; joint-pin relief and
conditional replay are the clearest examples.

Each source-backed mechanism changes at least one field of
\Cref{eq:live-information}. Transcript compression changes width and provenance;
hosting changes location and temporary custody; a lifecycle loan shortens the live interval;
recomputation replaces residency with a cleanup path; measurement-based
uncomputation changes cleanup and its phase proof duty; and hard-$Q$ metadata
replaces a full value with a narrower description whose reversal is more
expensive. The schema is not claimed as a complete ontology. A material
source-backed transition that cannot be represented without erasing an
important technical distinction would require it to be extended. Nonce and
parameter-only rows are search outcomes rather than contrary mechanism cases.

The order of discovery also becomes legible through this schema. Early in the
challenge, values and allocated locations were visible, while logical owner and
live interval remained implicit. Joint-pin analysis made ownership explicit;
transcript compression made provenance explicit; measured cleanup made quantum
phase part of the resource contract; low-$Q$ exploration made witness lifetime
explicit; and late carry release reduced progress to the last consumer of one
bit. The trajectory is therefore not a collection of isolated tricks, but a
progressive refinement of the circuit's information model.

\subsubsection{The Circuit-Improvement Search as a Damped Newton Descent.}
\label{sec:damped-newton}

It is tempting to read the open autoresearch effort for circuit improvement as discussed above as a greedy descent, in which each submission simply steps in whatever direction most reduces the objective. For an easy-to-evaluate, hard-to-solve problem, this reading is accurate only for the dense stretches of small local optimizations, and it is silent about the larger unblocks where most of the insight lives. The reason is that the feasible set of valid solutions is usually non-smooth and laced with constraints. In the {\challengename} case a single shared register can make a genuine reduction in width invisible, a residual phase can invalidate a solution that is otherwise numerically correct, and an algebraic shortcut can be worthless if the quantity it saves must remain live through the most expensive region. On such a surface the direction in which the score last improved, the first-order information, is not enough to decide where to go next.

A more faithful description is that the loop behaves, in a loose but useful sense, like a damped Newton method. A participant proposes a step, measures the residual with the evaluator and the score, inspects the source and the accumulated notes to learn which local constraint was actually binding or which apparent direction was in fact flat, and revises a working model of the frontier before stepping again. The relevant curvature is not a numerical Hessian but the discovered structure of the problem: in this challenge, which live quantities jointly own the peak, which intermediate windows must survive, and which cleanup obligations a given route commits to. The damping is supplied by the exact evaluator and the correctness contract, which hold back an attractive but unproven step, such as a gate cut that lowers the count or a slick algebraic identity, until its value, phase, and ancilla behavior have survived verification. Verification thus plays the role that a trust region plays in optimization, keeping the search from taking a confident step onto an infeasible point.

The consequence that generalizes beyond this problem is that failed proposals are not wasted searches. A rejected port, a candidate that a closer look reveals to hide a resource deficit elsewhere, or a note establishing that an apparent local saving was really a global side effect, each carries second-order information about the local geometry of the feasible set. Such results identify which directions are flat, which cross a constraint surface, and which are worth re-parameterizing, and they are exactly what make the accepted steps intelligible. An open autoresearch record that logs only its successes is therefore a curve without an explanation. Preserving negative results as first-class, shared artifacts is what lets the community build an increasingly accurate model of a hard feasible set, and it is a large part of why the collective search converges faster than any single greedy trajectory could.
