# Supplementary material for: ECDSA.Fail: Open Autoresearch for Optimizing Elliptic-Curve Point Addition in Shor's Algorithm
Source: arXiv:2609.09582 source file (2026-09-19)
Supplement: Supplementary file 2 [file 08-appendix-anatomy-of-optimization-techniques.tex]

\section{Anatomy of the Agent-Identified Quantum Circuit Optimizations}
\label{sec:anatomy}

\Cref{sec:optimization-technique-breakdown} classified the $400$ scored source
commits of the public competition into the nine optimization families and two
residual buckets of \Cref{fig:family-census-tree}. This appendix supplies the
mechanism-level anatomy behind that census: for each family, what the
transformation does to the reversible circuit, which correctness obligation
licenses it, which factor of the score $S=QT$ (\Cref{sec:cost}) it moves, and
which audited commits attest it. Where a family's marquee instance is already
developed in the main text---the Jump-2 Euclidean recurrence
(\Cref{sec:jump-two-gcd}), the base-$5$ transcript codec
(\Cref{sec:base-five-codec}), specialized Karatsuba squaring
(\Cref{sec:specialized-squaring}), register-shared Euclidean inversion
(\Cref{sec:register-shared-eea}), constant propagation (\Cref{sec:consprop}),
and dead-code elimination (\Cref{sec:dead-code-elimination})---we do not repeat
that treatment, and record only the technique's placement in the taxonomy, its
neighbouring mechanisms, and its commit-level record. The complete per-commit
ledger, with each commit's joined leaderboard score, frontier delta,
contestant, and date, is \Cref{tab:supp-census}.

The archive records landed source transformations more reliably than it records
who first conceived them. Accordingly, \emph{agent-identified} denotes
optimization episodes surfaced and developed in an agent-mediated workflow; it
does not assign exclusive agency, authorship, or novelty to a model. Human
direction, community exchange, and imported research remain part of the
provenance, and are separated from local implementation claims below.

\paragraph{Why these nine families.}
The organizing idea is that the scored artifact is, in effect, a compiled
straight-line reversible arithmetic program: a fixed schedule of modular
additions, multiplications, and inversions over $\mathbb{F}_p$ realized as
Toffoli-and-Clifford gates on a bounded qubit register. Read this way, the
transformations in the archive are recognizably related to moves a classical
optimizing compiler makes on such a program, and six families accordingly carry
familiar compiler labels: algorithmic substitution, strength reduction, fusion,
windowing (loop blocking with precomputation), constant propagation, and
dead-code elimination. The remaining three have familiar classical analogues but
are separated here because reversibility changes their objective or proof duty:
an \emph{uncompute strategy} family, because scratch must be returned to
$\ket{0}$ without residual phase; a \emph{register and scratch allocation}
family, because the location and lifetime of quantum data directly set peak
logical width; and a \emph{codec/encoding} family, because reversible decoding
and cleanup determine the time--space exchange when resident quantum state is
replaced by encoded metadata. The claim is thus not that classical compilers
lack allocation or encoding, but that these transformations acquire distinct
semantic and resource consequences in a reversible circuit.

This transformation axis is deliberately orthogonal to the two the main text
already used: the metric axis---which score factor a change primarily moves---and
the primitive axis---which building block it touched (adder, comparator, modular
multiplier, Kaliski inverse). Because each commit is assigned the single family
naming its \emph{dominant} transformation, the families are a single-label
characterization rather than a claim that the underlying mechanisms are
disjoint; a submission routinely bundles several---a width truncation co-tuned
with a nonce reroll, or a carry-fold gadget that at once removes gates,
substitutes a cheaper equivalent, and merges two adjacent operations---and the
assignment records only which of them is primary. This boundary was the
principal source of disagreement during a second audit, which prompted
reassignment of multi-mechanism entries; because the released census preserves
only the reconciled primary labels, not the paired pre-reconciliation labels, we
do not report an inter-rater reliability statistic. The audit left the
qualitative conclusions below unchanged. The taxonomy is likewise open rather
than closed: later eras of the search---still wider windowing and, most
concretely, a prospective \emph{representation / coordinate change} family
(coset, projective, or Kim wide-$r$ representations, characterized in
pre-competition research but with no landed competition instance)---may force
additional families. We order the subsections below by structural role rather
than by frequency, leading with the skeleton-defining windowing family.

\paragraph{Which commits each claim rests on.}
This appendix draws on both halves of the source history defined in
\Cref{sec:optimization-technique-breakdown}. The census of
\Cref{fig:family-census-tree} counts only the scored commits of the public
competition and is reconciled against the public ledger in
\Cref{sec:supp-census}; the technique-level discussion inside each family instead
draws mainly on the earlier pre-competition commits, where the mechanism first
becomes source-auditable.\footnote{The
per-commit Toffoli and peak-qubit figures quoted in the family subsections below
are source-reported local counts, typically measured on that technique's own
primitive or working tree at the pre-competition commit where it landed (as
recorded in the corresponding source audit), not the global operating points of
\Cref{tab:headline-operating-points}. The working-tree peaks these deltas sit
on---often in the low thousands of logical qubits---therefore differ from the
promoted submissions' headline widths, and most identifiers are pre-competition
development hashes; where a competition submission hash is quoted (e.g.,
\texttt{9a81017}), the figures are that submission's own operating point.}

\paragraph{Distinguishing gate removal from re-sampling.}
One classification boundary cannot be settled from the diff alone and requires
running the evaluator. Because the score averages \emph{executed} Toffoli over a
Fiat--Shamir sample that the submission's nonce selects (\Cref{sec:evaluator}),
and because the low-width routes contain measurement-conditioned Toffolis whose
execution is data-dependent, a submission can lower its score in two ways that
look identical on paper: by \emph{removing gates}, or by \emph{re-sampling} to a
luckier ``island'' on which the same gates execute fewer times. We separate them
by rebuilding each ambiguous submission and comparing its \emph{static}
Toffoli-gate count---after nonce-tail and explicit padding changes are
excluded---to its parent's. A static-count drop is evidence that the emitted
gate stream contains fewer Toffoli instructions, though the source diff is still
required to identify the responsible mechanism; equality is not sufficient to
establish re-sampling, because two circuit bodies can contain the same number of
gates under different controls, so we classify a lower executed average as
re-sampling only when the source and op-stream comparison also finds no
circuit-body change apart from the identity tail. Applied to the eleven commits
that a diff read alone had left \emph{neutral}, this test reclassified eight as
real gate reductions and one as verifier search; with a third padding-only
submission surfaced in the wider re-audit, exactly three submissions across the
full audit change no gate at all, each merely adjusting the injected
\texttt{DUMMY\_TOFFOLIS} padding rather than the circuit. Some reclassified
reductions are \emph{approximate} (a width truncation that errs on a
sub-permille fraction of inputs and validates only under a co-hunted island); we
count them under their gate-removing mechanism but flag the integrity concern in
\Cref{sec:limitations}.

\paragraph{A score-weighted view.}
The census counts how \emph{often} each family was the primary move; the recovered
leaderboard scores (\Cref{sec:supp-census}) also permit an accounting view of
realized frontier movement. Let $\Delta_i$ be the ledger's signed score change
for entry $i$, so an improvement has $\Delta_i<0$. The $70$ largest reductions
$-\Delta_i$ account for $91.6\%$ of the gross reduction across all $400$ scored
entries; excluding the one that merely zeroes the injected
\texttt{DUMMY\_TOFFOLIS} gates leaves $69$, whose sum is the denominator of the
percentages below. This is a bookkeeping decomposition of realized deltas, not a
counterfactual estimate of each mechanism's isolated effect: source commits can
bundle changes, and later deltas depend on inherited earlier structure.

Under that accounting rule, the four structural families---register/scratch
allocation, fusion, windowing, and uncompute strategy---receive
${\approx}60\%$ of attributed frontier improvement ($21\%$, $18\%$, $13\%$, and
$8\%$ respectively), across just $26$ of the $69$ included commits (under
$7\%$ of all scored commits). Register-lifecycle changes, boundary
\texttt{cswap}-merge fusions, the commit landing the two-jump inversion
base, and measurement-based comparator uncomputes are associated with realized
deltas of hundreds of millions of score points; the two-jump landing records a
delta of nearly one billion. The contrast between count and attributed delta is
sharpest for fusion and windowing, which are rare by count ($3.0\%$ and $2.0\%$
of scored commits) yet together receive nearly one third of the accounted
improvement. Dead-code and redundancy elimination receives $39\%$, consistent
with sustained late-stage tuning rather than a small number of step changes.
Conversely, the families that a lever-\emph{name} count makes look substantial
shrink under a diff audit and under weighting alike: algorithmic substitution
(\Cref{sec:fam-algorithmic-substitution}) is small on both axes, and the
codec/encoding and constant-propagation families receive essentially no delta
in this scalar-frontier accounting---their moves lie mostly on the low-width
Pareto branch (\Cref{sec:low-qubit-track}), are superseded, or rarely advance
the scalar incumbent.


\subsection{Windowing}
\label{sec:fam-windowing}

In the accepted-commit census (\Cref{fig:family-census-tree}), windowing is the
primary move in $8$ competition commits ($2.0\%$), led by the wholesale landing of
the two-jump inversion base and its \texttt{K2} refinements; the family opens
the anatomy because that small count carries the competition's largest single
frontier movement. The windowed modular shift described below is the census's
\emph{windowed carry/shift blocks} change-type---the primary move in the
remaining $5$ of these $8$ commits; the specific Solinas-shift commits detailed
below are first documented before the competition, while the same
windowed-shift primitive recurs as a competition primary move.

Windowing asks whether a batch of $w$ consecutive loop iterations can be
processed in one wider operation rather than step by step. Its closest compiler
analogy is loop blocking with precomputation: a run of the body is replaced by
an amortized operation controlled by a small input window. Two instances appear
in the audited archive; the first changes the implementation of the circuit's
dominant cost centre.

\paragraph{Two-jump ($K2$) inversion windowing.}
The family's largest instance re-blocks the circuit's dominant cost centre, the
modular inverse, so that each reversible iteration advances \emph{two} steps of
the binary-GCD recurrence rather than one; \Cref{sec:jump-two-gcd} develops the
construction, its macro-step invariant, and its fixed convergence budget. Read
as a taxonomy entry, it is a windowing move because the recurrence and the
returned inverse are unchanged and only the iteration boundaries move, which
makes it exact conditional on convergence and leaves the enclosing
point-addition schedule untouched; the saving lands on average executed Toffoli.
Unlike an earlier era's naive low-bit matrix-lookup form, which a matrix-cost
lower-bound test decisively closed as a moonshot, the comparator-aware two-step
synthesis \emph{landed}: it shipped as the \texttt{DIALOG\_GCD} route
(\texttt{src/point\_add/kaliski\_jump.rs}), a wholesale alternate inversion
implementation that became the accepted competition base at submission
\texttt{cddd5df} and was then refined by a long series of admitted submissions.
A representative refinement, \texttt{DIALOG\_GCD\_K2\_PAIR\_COMPRESS}
(submission \texttt{9a81017}), packs the six raw transcript bits of two
consecutive \texttt{K2} steps into five sidecar bits---the pair code of
\Cref{sec:base-five-codec}, licensed by a reachability constraint between one
step's shift bit and the next step's low branch bit; it is reported
validator-clean over all $9{,}024$ shots at $1{,}313$ logical qubits and
$1{,}536{,}923$ average executed Toffoli. Being an exact transcript re-encoding,
it is distinct from the iteration-bound truncations of
\Cref{sec:fam-dead-code-elimination} and in particular from the documented
approximate ``$396$-iteration'' redteam variant that this operating point
deliberately excludes.

\paragraph{Windowed modular shift.}
The archive's second windowing instance batches a no-op stretch of the Solinas
reduction that normalizes products modulo $p = 2^{256} - 2^{32} - 977$. That
reduction walks the set bits of $c = 2^{32}+977$, whose nonzero positions are
$\{0,4,6,7,8,9,32\}$, doubling and correcting at each step; between bit $9$ and
bit $32$ the loop performs $22$ consecutive
\texttt{mod\_double\_inplace\_fast} calls that reduce nothing, because no bit of
$c$ is set in that range, yet each still pays a full mod-$p$
double-and-correct. Submission \texttt{c702290} replaces that stretch with a
single classical shift-by-$22$ that captures the overflow into a fresh
\texttt{spill} register, one sparse windowed correction that adds
$\mathit{spill}\cdot c$ back at $c$'s set-bit positions, and a single final
conditional subtract; the swap-based shift itself costs no Toffoli, so the
saving in average executed Toffoli is exactly the cost of the per-iteration reduction
boundaries that are deleted. The substitution is exact rather than approximate
and survives the evaluator's reversibility and phase checks
(\Cref{sec:evaluator}) by a lifetime discipline: the classical correction flags
are threaded through to a matching \texttt{mod\_shift\_right\_by\_k} that
replays the same steps in reverse against the same qubits, so the reverse shift
exactly cancels the forward one---an earlier attempt, \texttt{579db56}, failed
the phase-garbage check precisely because it recomputed an independent inverse
instead. The same primitive was applied at all three Solinas call sites
(\texttt{c702290}, \texttt{de71b0f}, \texttt{d396bbc}), with a later refinement
(\texttt{0c6235f}) exploiting the pseudo-Mersenne structure directly.

Both instances leave their algorithm in place and only re-block its schedule,
which distinguishes windowing from its neighbours: fusion
(\Cref{sec:fam-fusion}) merges exactly two adjacent operations to delete one
load/unload boundary, strength reduction
(\Cref{sec:fam-strength-reduction}) holds the schedule fixed and swaps a single
operation for a cheaper equivalent, and algorithmic substitution
(\Cref{sec:fam-algorithmic-substitution}) swaps the underlying algorithm
outright.


\subsection{Algorithmic Substitution}
\label{sec:fam-algorithmic-substitution}

Under a diff-level audit this family is the primary move in only $2$ scored
source commits ($0.5\%$): a Karatsuba squarer backend swap
(\texttt{28fe2f2}) and a Karatsuba $x$-tail-square swap
(\texttt{b6d6f41}). The wired \emph{main} modular multiplier stays schoolbook
and Kaliski remains the sole inversion route for the entire competition---a
name-based count over-reports this family at $61$ ($15.3\%$) because dozens of
commits carry \texttt{\_KARATSUBA\_} / \texttt{fermat\_inv} lever names whose
backends are never wired (default-\texttt{false} flags,
\texttt{\#[cfg(test)]} scaffolds), while their real dominant move is dead-code,
register, or strength reduction. Both commits sit in the census's single
\emph{multiplier/squarer swap} change-type; the schoolbook conversions and
in-Kaliski reverts below predate the competition and have no primary-move
instance within it.

A substitution qualifies here only when the replacement is extensionally
identical over $\mathbb{F}_p$---it must return the same residue modulo
$p = 2^{256}-c$ for every admitted input, so that the enclosing point-addition
schedule is unchanged and the swap is invisible to the validator of
\Cref{sec:evaluator} apart from its gate count---which is why these swaps
primarily move average executed Toffoli rather than peak width.

\paragraph{Schoolbook (grid) multiplication.}
The baseline modular multiply is a Horner shift-and-add walk that performs
$O(n)$ full conditional modular additions---a comparator, a Cuccaro add, and a
Solinas reduction per bit of the multiplier. The schoolbook form instead builds
the $n\times n$ array of bit-products with cheap AND gates, accumulates them
into a single wide $2n$-bit register, and reduces modulo $p$ once at the end;
the two schemes return the identical product, so the choice is a per-site cost
decision, not a change to the arithmetic. The first squaring conversion
(\texttt{a85389c}) saved roughly $170{,}000$ average executed Toffoli per call,
and converting the remaining \texttt{build()} multiplies to schoolbook form
removed on the order of $624{,}000$ across five commits. The wide accumulator is
real ancilla, however, so this cheaper algorithm needs more live scratch and can
raise the peak-width factor of the score $S = QT$ (\Cref{sec:cost}) wherever two
such calls are simultaneously live in one closure.

\paragraph{Karatsuba multiplication.}
Karatsuba substitutes schoolbook's $O(n^{2})$ grid for the classical
three half-width-product recombination, an $O(n^{1.585})$ scheme that again
returns the identical product; \Cref{sec:specialized-squaring} gives the
squaring-specialized form that survives in the final circuit, whereas the
commits below are the earlier generic-multiplier swaps. Applied to all four
multiply sites (\texttt{cc427db}) it lowered average executed Toffoli from $4{,}927{,}684$ to
$4{,}680{,}924$, but its half-sum and cross-term registers add live scratch,
which sharpens the same width trade-off. Pushing Karatsuba into the three
multiply sites \emph{inside} the Kaliski closure---the highest-peak-qubit region
of the circuit---reduced Toffoli yet worsened the product, and \texttt{bc2f2a4}
reverted exactly those sites to a scratch-lean add\slash subtract schoolbook
variant, trading a modest Toffoli increase for a larger width reduction. The net
value at any given site is therefore decided jointly with the register-allocation
constraints of \Cref{sec:fam-register-allocation} and the operation-level
rewrites of \Cref{sec:fam-strength-reduction}, which supplied the add\slash
subtract schoolbook variant that won those in-Kaliski sites back.

The family's largest instance acts on the other cost centre, the modular
inverse: the whole-inverse jump/safegcd reformulation that computes the same
$v^{-1}\bmod p$ through a different recurrence. In its landed form that
reformulation batches two GCD steps per reversible iteration through a
precomputed transition, so we classify it under Windowing
(\Cref{sec:fam-windowing}, the $2$-jump route) and record it here only as this
family's boundary case, where a change of algorithm and a change of schedule
coincide.


\subsection{Dead-Code and Redundancy Elimination}
\label{sec:fam-dead-code-elimination}

This is the archive's most frequent primary move by a wide margin: $244$ of the
$400$ scored source commits ($61.0\%$). Comparator and register-width truncation,
iteration-count and threshold tuning, and fold and carry-truncation levers
dominate, with a small dead-gate census tail. Its prevalence reflects the
late-competition regime, after the circuit skeleton had stabilized and most
tuning removed exact redundancies or support-conditionally truncated rarely
exercised work.

\Cref{sec:dead-code-elimination} states the transformations themselves---the
self-inverse cancellations, the two inductive bit-range invariants that license
width truncation, and the exact and support-conditioned iteration bounds. This
subsection adds what the taxonomy needs: why the family is the only genuinely
dual-factor one, how its members split across two correctness models, and the
commit-level record behind each.

It is the taxonomy's genuine dual-factor family because a deleted loop
iteration removes both the nonlinear work inside it \emph{and} the registers
sized to the iteration count, so a single transformation can move average executed
Toffoli (\Cref{sec:cost}) and peak logical width at once. Its members span two
qualitatively different correctness models---\emph{exact} deletions redundant for
every admitted input, and a single \emph{probabilistic} deletion licensed only
over the validator's fixed instance support---and that distinction, not the size
of the saving, is what the ordering below foregrounds.

Mapped onto the census change-types: \emph{self-inverse cancellation} and
\emph{negation elision} below are the \emph{dead-gate/self-inverse removal}
bucket ($21$); \emph{comparator and register-width truncation} is the census's
single largest change-type ($149$); \emph{iteration truncation} (exact and
probabilistic) is \emph{iteration/threshold tuning} ($37$); and a
\emph{fold/carry truncation} tail---fold vents and carry-tail skips, not written
up separately here---accounts for the remaining $37$.

\paragraph{Self-inverse cancellation.} An involution wrapped around a helper
call---a negate/\allowbreak act/\allowbreak un-negate bracket---is removed by
inlining the helper's body for the sign already on hand, so both involutions
vanish from the gate stream rather than being paid for and cancelled at run time.
In the Kaliski inverse plumbing the two \texttt{mod\_neg\_inplace\_fast} calls
bracketing the pair-1 modular-inverse unadd were deleted this way
(\texttt{0340f24}, $8{,}584{,}680\to 8{,}583{,}660$ average executed Toffoli),
and the identical pattern on the pair-2 unadd followed one commit later
(\texttt{23d3fa0}).

\paragraph{Negation elision.} This reaches the same matched bracket from
upstream: rather than collapsing a bracket that already exists, it chooses the
operand order at a value's source that never produces the unwanted sign---feeding
Kaliski $Rx-Qx$ instead of $Qx-Rx$ and flipping the one downstream consumer's
add\slash subtract polarity to absorb the flip (\texttt{ee1743e},
$19{,}041{,}786\to 19{,}040{,}766$), then propagating a single negative-native
sign convention through the shared \texttt{kaliski\_forward} primitive so that a
negation running four times per point addition is removed once at the source
(\texttt{53a4aeb}, $19{,}040{,}766\to 19{,}038{,}718$).

\paragraph{Comparator and register-width truncation.} The family's single most
frequent move---$149$ of the $244$ dead-code submissions---narrows an operation
to the bits that can be nonzero rather than deleting a whole loop pass. Because
the two invariants of \Cref{sec:dead-code-elimination} between them cover the
whole iteration range, any operation touching bits outside the proven-nonzero
prefix is an identity paid for in full; the resulting rewrites narrow an adder to
its live prefix and drop a control whose two outcomes provably coincide (a
\texttt{cswap} chain of $n-1=255$ Toffoli-bearing Fredkin gates becoming free
swaps when $v_w[0]$ is zero on both branches, \texttt{e996391}). In the source
record these are the \texttt{COMPARE\_BITS}, \texttt{WIDTH\_MARGIN}, and
\texttt{KAL\_*\_TRUNC\_W} levers.

\paragraph{Iteration truncation.} Where width truncation narrows an operation,
iteration truncation removes whole loop passes, shrinking the gates \emph{and}
the counters and history registers indexed by the loop bound. The exact
$2n-1=511$ bound was established not by formal proof but by exhaustive search
over the $v=2^{k}$ stress class plus random and near-boundary sampling, treated
as sufficient because the harness re-checks classical correctness every
run---that single bound drops every iteration-indexed register by one
(\texttt{c46a010}), and the larger late-iteration truncations (for example
\texttt{afa876f}, $-259{,}080$ Toffoli) compose freely on top because each only
deletes work already scoped to be a no-op; skipping a provably-unreachable
Solinas correction is the same move. Every deletion in these paragraphs is exact
for all admitted inputs.

\paragraph{Probabilistic iteration truncation.} Pushing the same bound
\emph{below} its provable floor looks like the same move but changes the
correctness model, since a rare input requiring more iterations would silently
produce a wrong inverse. It is therefore not an all-input theorem but a
validation-support-conditioned claim, licensed only over the fixed Fiat--Shamir
instances the validator of \Cref{sec:evaluator} actually exercises and justified
by two support-conditioned ingredients rather than a proof: a cited
application-level tolerance argument that Shor's algorithm absorbs on the order
of one per-cent per-point-addition error~\cite{google26}, and the empirical
zero-failure sampling reported in \Cref{sec:dead-code-elimination}. Because it
also shrinks the iteration-indexed history registers, \texttt{5f2adb5} is a
genuine double win and among the family's largest single reductions on either
axis---yet its correctness lives entirely in how the truncation is justified:
tellingly, an earlier commit trying the identical numeric bound under a
\emph{deterministic}-correctness framing was reverted, while the same change
succeeded once presented as an explicit bounded-error claim.


\subsection{Register and Scratch Allocation}
\label{sec:fam-register-allocation}

This family is the primary move in $50$ submissions ($12.5\%$), spanning
scratch reuse, ancilla-lifetime, and in-place-mutation changes. A diff-level
audit finds it far more common than a lever-name count suggests because many
peak-qubit moves are recorded under arithmetic-sounding lever names. In census
terms, \emph{scratch reuse} is \emph{scratch/ancilla reuse} ($17$),
\emph{in-place mutation} is the like-named change-type ($3$), and
\emph{ancilla-lifetime windowing} is \emph{ancilla-lifetime / venting} ($30$,
the family's largest bucket). \emph{Horner evaluation} carries no census node
of its own: it is a multiplier-width streaming trick whose primary move is
counted elsewhere and is included here only for its mechanism.

This family is defined by changing the placement or lifetime of live storage,
so its primary target is $Q$, the peak logical width in $S=QT$
(\Cref{sec:cost}), rather than average executed Toffoli $T$. It is not the only
family capable of moving $Q$: codec, fusion, and windowing changes can do so as
well, and individual allocation changes can also alter $T$. The distinguishing
mechanism is that an allocation or lifetime change can lower a maximum without
removing a gate, provided it intersects every phase tied at that maximum. The
paragraphs below are the local, one-register instances of that mechanism; its
wholesale expression, in which complementary lifetimes let remainders, B\'ezout
coefficients, and quotient state share two physical work registers, is the
register-shared inversion of \Cref{sec:register-shared-eea}.

\paragraph{Scratch reuse.} The mildest move: when a fresh ancilla would be
allocated, borrow instead an in-scope register already provably at $\ket{0}$,
or replace a hand-rolled call site with the shared primitive that already
embodies the win. The correctness obligation is localized but not vacuous: the
borrowed register must enter and leave at $\ket{0}$, remain unaliased while in
use, and be restored before its owner returns. Handing
Kaliski step~1's \texttt{mcx3\_polar} scratch to the provably-zero \texttt{b\_f}
(\texttt{3e495b1}) or reusing \texttt{add\_f} at two more sites
(\texttt{8626f25}) elides alloc/free bookkeeping without altering a Toffoli,
while computing a shared sub-term once into a known-zero ancilla removes a
redundant compute/uncompute pair (\texttt{dfa4bd0}, \texttt{fb60dee}).

\paragraph{In-place mutation.} This refuses the copy entirely: a routine that
needs a negated, doubled, or offset version of a value it already holds walks
the live register through the whole transform and restores it exactly with the
inverse sequence, deleting the scratch copy, its copy-in and copy-out passes,
and its free. Correctness follows from the mutation being run with
\texttt{emit\_inverse}-derived exact inverses, so the round trip returns the
register to its entry value; aliasing the raw Kaliski inverse register into
\texttt{with\_kal\_inv} rather than copying it removes exactly one $n=256$-qubit
register from the peak (\texttt{419a4df}, $3339\!\to\!3083$), as does the
companion \texttt{sum\_y} deletion (\texttt{93cee90}, $3595\!\to\!3339$, both
$-256$). The same discipline can even pay to \emph{raise} the gate count:
walking the Karatsuba tail through $22$ in-place mod-$p$ doublings and their
inverse halvings rather than a shift-by-$22$ deletes the ${\sim}24$-qubit
spill/overflow/flag lane that alone bound the peak, buying a peak-width drop at a
small Toffoli cost (\texttt{fe29b53})---a register move precisely because it
resets $Q$, not $T$.

\paragraph{Horner evaluation.} This attacks the multiplier's live width by
streaming: an MSB-first multiply-accumulate doubles the accumulator it is
already touching rather than a separate scratch copy of the multiplicand, so the
intermediate products never all need to be resident at once and the whole
scratch register plus its double/halve restore walk disappears whenever the
accumulator is provably zero on entry. It is correct precisely because
``doubling the accumulator'' only preserves meaning when that accumulator starts
at $\ket{0}$, which is exactly the from-scratch multiply case, and the doublings
land on \texttt{acc} that the conditional adds already touch---no separate state
to restore (\texttt{b77a311}, $\sim\!130$k Toffoli per applicable multiply;
secondary strength-reduction membership).

\paragraph{Ancilla-lifetime windowing.} This addresses the high-water mark most
directly: a register whose declared scope spans a hot loop but which a
peak-driving section provably never touches---because an invariant holds it at
$\ket{0}$ or a known fixed value---is released across that section and
reallocated fresh afterward. The release is valid when the narrowing invariant
is established before the window and the register is
reallocated to a fresh $\ket{0}$ (and re-flipped to its fixed value if needed)
before its next use, changing no gate. Freeing \texttt{v\_w} across the
multiplication-heavy \texttt{body} on this argument (\texttt{1fd2656},
$3478\!\to\!3222$) is the single largest qubit reduction in its scan range,
again an $n=256$-qubit drop at zero Toffoli cost.

\subsection{Codec / Encoding}
\label{sec:fam-codec}

Classical systems also compress state; this family is separated because a
reversible codec must provide a coherent decode, use, and cleanup path while
trading resident quantum state for encoded metadata. It therefore spends
Toffoli to buy back peak qubits. Its $7$ census submissions ($1.8\%$) are all
the single \emph{trailmix / K5 codec} change-type, and its landed instance in the
scoring circuit is the base-$5$ transcript codec of \Cref{sec:base-five-codec},
whose proof obligations---support preservation, exact decoding, and complete
ancilla and phase cleanup---are exactly those that distinguish this family from
classical compression.

What places the family at the taxonomy's edge is that its most aggressive
expression pushes the same trade wholesale: rather than keep the full
transcript, quotient, and route values of the point-addition walk live in
registers, an encoding packs them into a compact per-step description and
reconstructs each value on demand, so far fewer qubits stay resident across the
peak. This is the extreme end of the register-and-scratch-allocation
spectrum---where scratch reuse borrows one known-zero register and windowing
frees one at its true last use, the codec converts whole classes of resident
arithmetic state into narrower encodings whose reversal must be replayed---and it
is the mechanism behind the low-width track's lowest-admitted-width artifact,
\texttt{b6f2b0a} at $825$ qubits, which correspondingly pays $489{,}161{,}900$
average executed Toffoli (\Cref{tab:admitted-pareto},
\Cref{sec:low-qubit-track}).\footnote{The source record attests the codec
mechanism directly---a \texttt{trailmix\_ludicrous/codec.rs} module (submission
\texttt{bdb1d22}) and a family of $K5$ tail/head compressors that pack per-step
raw state into fewer physical qubits---but the $825$/$489{,}161{,}900$ figures
are the \emph{artifact}'s operating point (\Cref{sec:results-summary},
\Cref{tab:admitted-pareto}), not a codec-specific measured delta; we attribute
the artifact to this mechanism, not a particular qubit or Toffoli saving to the
codec in isolation.} The trade is the steep reversible time--space exchange
\cite{bennett89,buhrman01} read through a single factor: the codec buys
reductions in $Q$ by spending in $T$, and the exchange rate steepens once
metadata and denominator-witness lifetime, rather than ordinary scratch, become
the binding constraint.


\subsection{Fusion}
\label{sec:fam-fusion}

Fusion, the primary move in $12$ submissions ($3.0\%$),
merges two \emph{adjacent} operations so that the load/unload or
compute/uncompute boundary each would pay independently need never be
materialized; the intervening body is left untouched, so the family moves average
executed Toffoli rather than peak width. Of the paragraphs below, the first three
are the census's \emph{gate/op fusion} change-type ($7$ submissions) and the
fourth, \emph{boundary cswap-merge}---collapsing two adjacent controlled swaps to
delete one load/unload boundary---is the primary move in the remaining $5$.

\paragraph{Comparator conjugation.}
The recurring shape is a self-inverse comparator called twice---once to compute a
flag, once to uncompute it---bracketing the caller's body, so the palindromic
MAJ-only sweep runs forward and inverse twice for $4n$ Toffoli where $2n$ of
carry-chain work is actually done. At \texttt{34c64b9} the step-2 ``greater-than''
comparator is folded into a single conjugation---one forward MAJ sweep, read the
carry, run the body inline, read the carry again to clear the flag, one inverse
sweep---so that $2n$ Toffoli suffice ($2{,}096{,}640$ fewer). The identical
rewrite of the zero-test comparator at \texttt{b655093} removed a further
$2{,}087{,}232$.

\paragraph{Shared-operand scratch fusion.}
When two adjacent arithmetic operations share an operand, the load and unload of
their common scratch register can be collapsed rather than paid twice. At
\texttt{90775e2}, Kaliski step~4's two conditional Cuccaro calls---a subtract of
$u$ from $v_w$ then an add of $r$ into $s$, both gated by the same
control---were fused around one \texttt{tmp} register, the in-place transform
$\texttt{tmp}\mathrel{\oplus}=\mathit{add\_f}\wedge(u\oplus r)$ reshaping the
loaded value into what the second operation needs instead of unloading and
reloading it ($524{,}288$ fewer Toffoli).

\paragraph{Branch collapse.}
Fusion can also merge an unconditional pass with its own conditional undo. At
\texttt{c413d6d}, the fast Solinas reduction's unconditional add of the constant
$c$ followed by a conditional un-subtract---in effect both branches of an
\texttt{if}/\texttt{else}---collapse to a single conditional add once the
post-shift overflow bit is recognized as the correction control ($655{,}864$
fewer). The move is order-sensitive: the paired-addition fusion at
\texttt{0bede51}, which loads the classical constant $Q_x$ once and doubles it in
place rather than loading it twice, became profitable only \emph{after}
\texttt{c413d6d} had made in-register doubling cheap.

\paragraph{Boundary cswap-merge.}
The recurring shape is a pair of width-$n$ controlled swaps in each Kaliski
iteration: step~3 orients the working registers, and step~9 commits the branch
decision. Each of the two GCD channels therefore pays $2n$ Toffoli per
iteration on swaps alone. The Fredkin identity
$\mathrm{cswap}(p)\cdot\mathrm{cswap}(q)=\mathrm{cswap}(p\oplus q)$ lets an
iteration's step-9 swap be deferred and merged with the \emph{next} iteration's
step-3 swap: a single persistent ``frame'' parity qubit carries the deferred
control $a_k$ across the iteration boundary, the merged swap is driven by the
combined parity $a_k\oplus a_{k+1}$ formed with a free CX, and the two width-$n$
swaps collapse to one plus a constant-size parity fix-up. Reversibility requires
the backward pass to mirror the same deferral, so the frame qubit is cleared at
the boundary that set it; because it is allocated only over that short span and
is never live during the step-4 peak, the merge is peak-neutral and moves only
average executed Toffoli.
At \texttt{d35d6e7} the construction was wired on the $(r,s)$ channel for
roughly $274{,}000$ fewer executed Toffoli, the largest single fusion win of
the competition. Commit \texttt{112d5a4} then extended the identical mechanism to the
$(u,v_w)$ channel, restricted to a $254$-iteration safe prefix. Beyond that
prefix, the cheap parity correction is no longer provably valid because
$u=v_w$ can occur near the walk's terminus. The remaining submissions in this
pattern only re-search that safe-iteration bound, leaving the mechanism
unchanged.

Fusion is strictly a one-adjacent-pair transformation: unlike its neighbours in
\Cref{sec:fam-windowing}, it keeps both operations and removes only the seam
between exactly two of them.


\subsection{Strength Reduction}
\label{sec:fam-strength-reduction}

A diff-level audit finds strength reduction as the \emph{primary} move in $14$
scored competition source commits ($3.5\%$)---equivalent-but-cheaper operation swaps
(negate-then-add, Solinas and \textsc{naf} folds, fast-adder reroutes) that keep
the algorithm's schedule intact---so it carries a node in
\Cref{fig:family-census-tree}. It was nonetheless chiefly a pre-competition family,
and the techniques below are drawn from that earlier record, where each
mechanism first becomes source-auditable. Of the census's two change-types,
\emph{fast-adder reroute} ($9$) is \emph{Fast-adder substitution} below and
\emph{solinas / NAF fold} ($5$) covers \emph{Solinas reduction} and
\emph{signed-digit constant decomposition}; \emph{negate-add substitution} and
the \emph{Litinski add-subtract} row are pre-competition techniques with no
primary-move instance during the competition.

Where algorithmic substitution (\Cref{sec:fam-algorithmic-substitution}) swaps
one primitive for a different one, strength reduction keeps the schedule of
modular operations intact and replaces a single operation with a provably equal
but cheaper reversible realization; the win is invisible to the abstract
arithmetic but decisive for the gate count, and it moves average executed
Toffoli rather than peak width (\Cref{sec:cost}).

\paragraph{Solinas reduction.}
Because secp256k1's modulus is $p = 2^{256} - c$ with $c = 2^{32} + 977$ a
small, sparse $33$-bit constant, any $T \in [0, 2p)$ satisfies $T \bmod p
= (T \bmod 2^{256}) + c$ whenever the top-bit overflow fires (i.e.\ $T \ge 2^{256}$), so reduction needs only a
conditional correction by the small, sparse $c$ controlled by a single overflow
bit rather than a full comparison and subtraction against the dense $256$-bit
$p$. Inlining that add-$c$/branch/parity pattern into Kaliski's step~8
(\texttt{3536f4c}) removes $2{,}090{,}712$ Toffoli. The rewrite is bit-identical
because the reduction predicate is exactly the shifted-out top bit and, in the
doubling case, the correction flag is uncomputed for free by parity, since the
input was just doubled and $p$ is odd; the companion single-add refinement that
collapses the speculative add-then-undo pair is the branch collapse of
\Cref{sec:fam-fusion}.

\paragraph{Negate-add substitution.}
The identity $acc - X \equiv acc + (p - X) \pmod p$ is free algebraically, but a
conditional modular subtractor carries a comparator and underflow-correction
pass that the conditional adder does not---$1{,}536$ versus $1{,}280$ CCX per
iteration in this circuit's schoolbook multiplier---so the technique negates the
subtrahend once, drives the inner loop with the cheaper add primitive, and
negates back. Applied to the hottest inner loop \texttt{mod\_mul\_sub\_qq}
(\texttt{a462064}), this removes $256{,}016$ Toffoli, a fixed one-time cost
amortized against a per-iteration saving over a $256$-bit multiply. The computed
residue is unchanged because $p - X$ is $X$'s exact modular negation and the
loop reconstructs the identical accumulator.

\paragraph{Signed-digit constant decomposition.}
Multiplying a register by a fixed classical constant costs one Cuccaro add per
set bit, so recoding the Solinas correction constant $977 =
0\mathtt{b}1111010001$ (six set bits) as the four-term signed expression $977 =
2^{10} - 2^{6} + 2^{4} + 2^{0}$ collapses the contiguous run $\{6,7,8,9\}$ into a
single $2^{10} - 2^{6}$ pair and shortens the operation list without touching
the algorithm or the registers (\texttt{b1d04b7}, then \texttt{a0b7de6} at the
outer Solinas loop). Since a Cuccaro subtraction is merely the inverse gate
sequence of an addition and costs the same, and the shift's reverse is updated
symmetrically with flipped signs, the recoded constant computes the identical
product.

\paragraph{Litinski add-subtract schoolbook.}
This variant replaces each schoolbook row's AND-compute-then-add construction
with a single controlled two's-complement add-subtract row. The former costs
$2n{-}1$ Toffoli; the latter costs $n{-}1$ and needs no separate AND row,
roughly halving the per-row cost. Laid inside the
half-width inner multiplies of $1$-level Karatsuba (\texttt{28737ac}), it is the
largest single Toffoli reduction in its scan range ($333{,}794$, from
$4{,}672{,}931$ to $4{,}339{,}137$), at a modest peak-width cost ($+107$ qubits)
from the wider $(2n{+}1)$-bit accumulator. The row still evaluates $x\cdot y$
exactly: the controlled add-subtract layering produces $2xy$ plus a fixed
algebraic correction that is divided out by relabeling bits.

\paragraph{Fast-adder substitution.}
Swapping an ancilla-lean in-place Cuccaro adder for the pre-existing
carry-ancilla ``fast'' variant shortens the gate-count-bearing path at five
call sites in \texttt{mod\_shift\_left/right\_by\_k} (\texttt{384ed8a}: $-17{,}400$
Toffoli for $+21$ peak qubits). Because it buys Toffoli back with qubits, it is
a strength reduction only when peak width has local headroom---the commit's own
check confirms the transient peak stays below the enclosing Solinas
\texttt{mod\_add\_qq\_fast} peak---so this is a boundary case whose secondary
membership is in register allocation (\Cref{sec:fam-register-allocation}). The
two adder variants compute the identical sum; only their scratch footprint and
critical path differ.


\subsection{Constant Propagation and Classical Specialization}
\label{sec:fam-constant-propagation}

This family is the primary move in $19$ competition source commits ($4.8\%$), all
of the host-derived classical-specialization kind: commits that recognize a
value as classically fixed on the validator-supported path and specialize or
host it accordingly. The two named techniques below were established before the
competition, but---unlike strength reduction, which largely receded once it
began---classical specialization remained a live \emph{primary} lever
throughout, which is why its competition-era count is substantial. Both techniques below are the census's single \emph{host-derived /
classical specialization} change-type ($19$).

This family collects the transformations that exploit a value the circuit
already knows classically---a fixed multiplier bit, a compile-time offset, or a
loop branch that is provably forced on every admitted input---to specialize or
simply skip reversible work; because the exploited value is genuinely fixed, the
specialized circuit answers the validator of \Cref{sec:evaluator} on every
admitted instance exactly as the general one would, and the saving lands on the
average-executed-Toffoli factor (\Cref{sec:cost}) at unchanged peak width.

\paragraph{Classical conditioning.}
The family's primitive move---specializing a sub-circuit on a multiplier bit
that is classical for the evaluation instance rather than held in
superposition---is called \emph{Constprop} in the source record and is developed
in \Cref{sec:consprop}.

\paragraph{Guaranteed-prefix specialization.}
The family's larger instance applies the same specialize-on-a-known-predicate
idea to an entire loop prefix rather than a single gate, and in doing so it
borrows from algorithmic substitution
(\Cref{sec:fam-algorithmic-substitution}) as a secondary character. Kaliski's
binary almost-inverse (\Cref{sec:fam-algorithmic-substitution}) terminates when a
sum invariant reaches a target value; for $256$-bit \texttt{secp256k1} inputs
that invariant starts above $2^{255}$, so a minimum-step-count argument shows the
loop \emph{cannot} terminate during its first several iterations for any nonzero
input. Those leading iterations therefore always take the same non-terminating
branch, and the general branch-covering machinery a generic
\texttt{kaliski\_iteration} must carry is dead weight there. The optimization
replaces that guaranteed-nonterminal prefix with a bespoke branch-free primitive
(\texttt{kaliski\_iteration\_bulk\_prefix3}), proven classically equivalent to the
generic body restricted to the forced branch---by a companion
\texttt{kaliski\_equiv.rs} module checked against sampled reachable states, with
a mirrored backward step---\emph{before} it is wired into the live
forward/reverse passes. Its rollout was staged: \texttt{e80edd9} first landed the
specialized steps behind an opt-in flag (\texttt{KAL\_BULK3\_EXPERIMENT}),
leaving the scored build untouched, and \texttt{91fe506} then enabled the
prefix by default while extending the proven-safe span to $304$ iterations,
moving the scored circuit from $4{,}394{,}546$ to $4{,}236{,}292$ average
executed Toffoli ($-158{,}254$, or $3.6\%$) at unchanged width; \texttt{a25978e}
later restored that default on top of a $511$-iteration robustness baseline and
recovered the identical figure. Because the replaced iterations are proven
identical to the generic body on \emph{all} reachable nonzero inputs, this is a
guaranteed-prefix argument and not the empirical, support-selected truncation of
\Cref{sec:fam-dead-code-elimination}, and it does not narrow the admitted input
set.

\subsection{Uncompute Strategy}
\label{sec:fam-uncompute-strategy}

Uncompute strategy is the primary move in $22$ submissions ($5.5\%$, all measurement uncompute)---a diff-level audit finds it far more common than a lever-name count reports, because measurement-based clears (\texttt{hmr}/\texttt{cz\_if}) are invisible in the commit subject and surface only in the diff; and the choice it governs is additionally exercised in almost every submission, because reversibility is not optional. All $22$ census submissions are \emph{measurement uncompute}---the \emph{Measurement-based uncompute} paragraph below; the other four strategies are the compute--uncompute / Bennett discipline that reversibility forces on almost every submission but that is rarely itself the scored primary move.

Every scratch value must return to $\ket{0}$ or the run fails the reversibility
check of \Cref{sec:evaluator}, so the question this family answers is never
\emph{whether} to uncompute but only \emph{how}; the factor its choices move is
average executed Toffoli, and the units below are the menu of ways to avoid
paying the reverse sweep in full.

\paragraph{Ancilla-clean uncompute.}
The baseline discipline is compute--copy--uncompute: compute an intermediate
into fresh scratch, copy the wanted result out with a single \texttt{CX}, then
replay the computation in reverse to drive every ancilla back to $\ket{0}$
before freeing it. This roughly doubles the gate count of the forward
computation and is the $\sim\!2\times$ price that replaces a banned
\emph{dirty free}: once the harness's strict-reset check began panicking on any
nonzero free (\texttt{dc8fe9d}), primitives that had ``passed'' by dirty-freeing
a still-set ancilla had to be honestly rebuilt, as when \texttt{cmp\_neq\_zero}
was re-expressed as a palindromic de-Morgan OR chain with an explicit reverse
sweep (\texttt{266f418}). Every strategy below is an attempt to pay less than
this full reverse sweep.

\paragraph{Compute--act--uncompute (Bennett conjugation).}
Rather than hand-write the reverse sweep, this strategy brackets an action
between a compute block $C$ and its exact inverse $C^{-1}$ and makes $C^{-1}$
mechanical: an \texttt{emit\_inverse}/\texttt{conjugate} helper records the
forward block's gate stream, re-emits it reversed, and panics on any
non-invertible op, so the teardown can never drift out of sync with the setup
(\texttt{fe8875a}, which introduces the \texttt{emit\_inverse}/\texttt{conjugate}
helpers and rebuilds \texttt{cmod\_halve} as the exact inverse of \texttt{cmod\_double}). The trade-off is that the reverse is
generated for free but is only ever the recorded gates played backward---it can
never substitute a cheaper equivalent reverse.

\paragraph{Emit-inverse.}
The same machinery can define an entire standalone primitive as the mechanical
gate-inverse of its partner---subtract from add, halve from double---whenever
the forward primitive is already clean, since a clean reversible circuit's own
gate-level inverse is correct by construction. Defining
\texttt{mod\_sub\_qq} as \texttt{emit\_inverse(mod\_add\_qq)} (\texttt{dad5057})
removed a hand-written negate--add--negate triplet, lowering executed Toffoli
from $101{,}284{,}162$ to $98{,}893{,}282$ and, by deleting the \texttt{tmp}
register that triplet needed to reconstruct its own operand, cutting peak width
from $3{,}595$ to $3{,}339$ ($-256$ qubits)---the rare uncompute move that helps
both factors of $S=QT$ (\Cref{sec:cost}) at once. Its limitation is intrinsic:
\texttt{emit\_inverse} can only replay recorded gates backward, so the moment a
cheaper non-gate-reversal inverse exists (\texttt{8212f6b}) it becomes a
ceiling and the reverse must be hand-written outside the mechanism.

\paragraph{Measurement-based uncompute.}
When a scratch ancilla holds an isolated AND product that is provably unchanged
at the point it must return to $\ket{0}$, Gidney's trick replaces the second
Toffoli of the textbook uncompute with a Hadamard-measure-reset (\texttt{Hmr})
and a single classically-conditioned \texttt{CZ} on the two original controls,
at $0$ Toffoli per bit rather than one. The cost moves off the gate-count axis
onto a measurement plus a feed-forward classical bit---favourable under a
validator that scores executed Toffoli---but only after the surrounding gadget
is restructured so the AND product lives in its own qubit; applied to a
dedicated Cuccaro carry lane it halves the adder from $2(n{-}1)$ to $(n{-}1)$
Toffoli in a single commit (\texttt{8d54b18}). Because \texttt{Hmr} is not a
deterministic gate \texttt{emit\_inverse} can capture and replay, this strategy
is mutually exclusive with emit-inverse: reaching for it inside a
machine-generated reverse forces that backward pass to be hand-written first
(\texttt{8212f6b}).

\paragraph{Bennett pairing.}
The last strategy attacks not the cost of one uncompute but how many times an
expensive one runs: when a value-mutating, self-restoring routine that is
itself internally a Bennett pair is called twice back to back---once to
transform an input in place and use it, once purely to restore it---the inner
loop executes four times. Computing the transform into a fresh output register
while leaving the input live, then uncomputing only that output, folds two
conjugation pairs into one and roughly halves the loop executions without
widening the peak, since the scratch footprint is reused sequentially rather
than duplicated. Folding the Kaliski almost-inverse's two call sites this way
(\texttt{3af7f42} and the symmetric \texttt{408174a}) produced the largest
single Toffoli reductions in the corpus ($98{,}887{,}162\to77{,}082{,}106$ and
$77{,}082{,}106\to55{,}277{,}050$, each $-21{,}805{,}056$), and holding the
Kaliski state live across the caller's body (\texttt{8e0c9f6}) removed another
wrapped forward-and-reverse pass ($31{,}642{,}202\to20{,}608{,}890$).
