# Supplementary material for: ECDSA.Fail: Open Autoresearch for Optimizing Elliptic-Curve Point Addition in Shor's Algorithm
Source: arXiv:2609.09582 source file (2026-09-19)
Supplement: Supplementary file 3 [file 09-appendix-census-of-source-commits.tex]

\section{Optimization Census of Accepted Competition Source Commits}
\label{sec:supp-census}

\benhuang{Working on this atm}

\jieyi{Gather the raw Claude/Codex prompt sessions from the participants. Add the sanitized version to Github, and provide a high-level overview here.}

This appendix lists every accepted source commit of the public competition
(\Cref{sec:anatomy}), assigned to its primary transformation family or residual
bucket---the same census summarized in \Cref{fig:family-census-tree}, here
expanded to one row per commit. Official operating points---\emph{Score}~$=$
average executed Toffoli $\times$ peak qubits (lower is better) and $\Delta$, the
score change versus the prior public frontier---are joined from the ecdsafail
leaderboard; they are not in the git history itself. Of the $404$ accepted
``Accept submission'' commits through 18 July, $400$ have leaderboard score
records: $397$ match the \texttt{promoted} rows in the 2 July ledger snapshot
used for the headline operating points, and three are later scored commits. The
remaining four are the contest's \texttt{DUMMY\_TOFFOLIS} bootstrap commits,
which went through the acceptance plumbing but were never scored and are marked
\emph{(unscored)}. Accepted source commits and current ledger-status rows are
therefore related archival views, not interchangeable counting units. Each
row's assignment is made by an audit of its actual \texttt{git show} diff (not
its commit subject or lever name, which are frequently unreliable), matching
\Cref{fig:family-census-tree}. Rows are grouped by family
in descending order of frequency---with the two residual buckets (verifier
search, neutral) and the unscored bootstrap group placed last---then by
change-type (level~2 of \Cref{fig:family-census-tree}), and within a change-type
by score (best first).

The largest recorded frontier delta belongs to the two-jump inversion base
(\texttt{cddd5df}, under Windowing), whose $\Delta$ is nearly one billion; it is the landed
\texttt{DIALOG\_GCD} reimplementation of the modular inverse. This ledger lists
all $404$ accepted commits, including the four unscored bootstrap rows---placed
in their own \emph{Unscored bootstrap} group---that \Cref{fig:family-census-tree}
excludes; on the $400$ scored source commits the ledger and the figure agree family
by family.

{\small
\setlength{\tabcolsep}{4pt}
\begin{longtable}{@{}lllrr@{}}
\caption{Competition optimization census: all $404$ accepted source commits
(\#883--1294) through 18 July, classified by primary family,
with official leaderboard score and frontier delta where available. $400$
scored; $4$ unscored bootstrap commits.}\label{tab:supp-census}\\
\toprule
\textbf{Commit} & \textbf{Contestant} & \textbf{Date} & \textbf{Score} & \textbf{$\Delta$}\\
\midrule
\endfirsthead
\multicolumn{5}{@{}l}{\small\itshape \Cref{tab:supp-census}, continued}\\[2pt]
\toprule
\textbf{Commit} & \textbf{Contestant} & \textbf{Date} & \textbf{Score} & \textbf{$\Delta$}\\
\midrule
\endhead
\midrule
\multicolumn{5}{r@{}}{\small\itshape continued on next page}\\
\endfoot
\bottomrule
\endlastfoot
\addlinespace[2pt]
\multicolumn{5}{@{}l}{\rule{0pt}{2.6ex}\textbf{Dead-Code and Redundancy Elimination}~\small(244)}\\[1pt]
\multicolumn{5}{@{}l}{\quad\itshape comparator/width truncation \small(149)}\\
\texttt{75851e6} & bket7 & 2026-06-19 & $1{,}658{,}362{,}156$ & $-319{,}484$\\
\texttt{57eb64b} & benhuang2025 & 2026-06-19 & $1{,}669{,}072{,}000$ & $-3{,}061{,}328$\\
\texttt{1caf521} & mpjunior92 & 2026-06-16 & $1{,}672{,}963{,}776$ & $-1{,}569{,}792$\\
\texttt{7bab51f} & nasqret & 2026-06-14 & $1{,}677{,}861{,}900$ & $-498{,}420$\\
\texttt{f50ae3b} & gnuchev & 2026-06-14 & $1{,}678{,}360{,}320$ & $-269{,}100$\\
\texttt{6878ef8} & gnuchev & 2026-06-14 & $1{,}678{,}629{,}420$ & $-319{,}410$\\
\texttt{cf99209} & nasqret & 2026-06-13 & $1{,}683{,}083{,}736$ & $-526{,}864$\\
\texttt{186d9d7} & rubenmarcus & 2026-06-12 & $1{,}699{,}653{,}032$ & $-767{,}774$\\
\texttt{6777223} & rubenmarcus & 2026-06-12 & $1{,}700{,}420{,}806$ & $-627{,}298$\\
\texttt{0d1d1e7} & mpjunior92 & 2026-06-12 & $1{,}701{,}048{,}104$ & $-293{,}062$\\
\texttt{8cd8104} & jackylee0424 & 2026-06-11 & $1{,}702{,}054{,}020$ & $-1{,}013{,}749$\\
\texttt{5a783e4} & nasqret & 2026-06-11 & $1{,}704{,}784{,}725$ & $-270{,}945$\\
\texttt{f4404de} & jackylee0424 & 2026-06-11 & $1{,}713{,}097{,}160$ & $-26{,}840$\\
\texttt{1a5e620} & BitWonka & 2026-06-10 & $1{,}716{,}174{,}108$ & $-26{,}999{,}973$\\
\texttt{00fb66d} & jieyilong & 2026-06-10 & $1{,}743{,}174{,}081$ & $-623{,}931$\\
\texttt{707c1d9} & jieyilong & 2026-06-10 & $1{,}765{,}489{,}770$ & $-632{,}220$\\
\texttt{8e0bf4f} & BitWonka & 2026-06-10 & $1{,}766{,}121{,}990$ & $-2{,}044{,}435$\\
\texttt{ab5469b} & jackylee0424 & 2026-06-10 & $1{,}774{,}726{,}350$ & $-20{,}560$\\
\texttt{980ed3a} & jackylee0424 & 2026-06-09 & $1{,}785{,}547{,}335$ & $-1{,}286{,}285$\\
\texttt{2dcf00d} & jackylee0424 & 2026-06-08 & $1{,}820{,}641{,}701$ & $-28{,}534$\\
\texttt{f3820d0} & SamrendraS & 2026-06-08 & $1{,}823{,}175{,}078$ & $-1{,}406{,}122$\\
\texttt{da55bbb} & SamrendraS & 2026-06-08 & $1{,}824{,}581{,}200$ & $-694{,}200$\\
\texttt{73f4f48} & gnuchev & 2026-06-08 & $1{,}891{,}349{,}200$ & $-1{,}475{,}700$\\
\texttt{a5a590a} & gnuchev & 2026-06-08 & $1{,}892{,}824{,}900$ & $-109{,}934$\\
\texttt{94927be} & jackylee0424 & 2026-06-07 & $1{,}893{,}823{,}629$ & $-3{,}142{,}197$\\
\texttt{013f1f7} & zuiris & 2026-06-07 & $1{,}899{,}562{,}014$ & $-1{,}666{,}560$\\
\texttt{99b9cff} & zuiris & 2026-06-07 & $1{,}901{,}228{,}574$ & $-4{,}775{,}252$\\
\texttt{fc84586} & jackylee0424 & 2026-06-07 & $1{,}911{,}704{,}516$ & $-676{,}508$\\
\texttt{8925623} & BitWonka & 2026-06-07 & $1{,}939{,}751{,}375$ & $-188{,}208$\\
\texttt{779fc2b} & jackylee0424 & 2026-06-06 & $1{,}944{,}384{,}690$ & $-677{,}026$\\
\texttt{ace6347} & teddyjfpender & 2026-06-06 & $1{,}945{,}061{,}716$ & $-661{,}342$\\
\texttt{e0767c7} & jackylee0424 & 2026-06-06 & $1{,}945{,}723{,}058$ & $-677{,}026$\\
\texttt{3033d01} & jackylee0424 & 2026-06-06 & $1{,}967{,}891{,}695$ & $-675{,}444$\\
\texttt{88079e6} & 10d9e & 2026-06-06 & $1{,}969{,}242{,}583$ & $-675{,}444$\\
\texttt{8e13587} & runeape-sats & 2026-06-06 & $1{,}969{,}918{,}027$ & $-141{,}372$\\
\texttt{ebbe44e} & zuiris & 2026-06-06 & $1{,}977{,}629{,}346$ & $-827{,}329$\\
\texttt{7f656bd} & zuiris & 2026-06-06 & $1{,}978{,}786{,}502$ & $-4{,}018{,}630$\\
\texttt{1121d80} & welttowelt & 2026-06-06 & $1{,}982{,}805{,}132$ & $-1{,}361{,}360$\\
\texttt{cee4044} & welttowelt & 2026-06-06 & $1{,}984{,}166{,}492$ & $-1{,}511{,}895$\\
\texttt{c80fc1c} & newjordan & 2026-06-06 & $1{,}990{,}208{,}636$ & $-1{,}123{,}928$\\
\texttt{974689f} & newjordan & 2026-06-06 & $1{,}991{,}332{,}564$ & $-680{,}134$\\
\texttt{373fb4d} & newjordan & 2026-06-06 & $1{,}992{,}012{,}698$ & $-680{,}134$\\
\texttt{9906ec0} & newjordan & 2026-06-06 & $1{,}992{,}692{,}832$ & $-443{,}794$\\
\texttt{2f1f175} & newjordan & 2026-06-06 & $1{,}993{,}136{,}626$ & $-680{,}134$\\
\texttt{196d830} & newjordan & 2026-06-06 & $2{,}013{,}389{,}651$ & $-1{,}397{,}032$\\
\texttt{22624a0} & BitWonka & 2026-06-06 & $2{,}014{,}786{,}683$ & $-1{,}150{,}188$\\
\texttt{587b6d8} & anshu4321 & 2026-06-06 & $2{,}015{,}936{,}871$ & $-680{,}134$\\
\texttt{4ef0046} & BitWonka & 2026-06-05 & $2{,}016{,}617{,}005$ & $-212{,}706$\\
\texttt{02049b8} & 10d9e & 2026-06-05 & $2{,}016{,}829{,}711$ & $-1{,}150{,}188$\\
\texttt{91061af} & newjordan & 2026-06-05 & $2{,}020{,}184{,}357$ & $-1{,}838{,}686$\\
\texttt{5ad4427} & newjordan & 2026-06-05 & $2{,}022{,}023{,}043$ & $-1{,}688{,}320$\\
\texttt{58ecf0a} & 10d9e & 2026-06-05 & $2{,}025{,}245{,}640$ & $-633{,}600$\\
\texttt{351a0d0} & 10d9e & 2026-06-05 & $2{,}025{,}879{,}240$ & $-1{,}151{,}040$\\
\texttt{83da96f} & 10d9e & 2026-06-05 & $2{,}027{,}030{,}280$ & $-3{,}429{,}360$\\
\texttt{ec0fa98} & 10d9e & 2026-06-05 & $2{,}030{,}459{,}640$ & $-2{,}808{,}960$\\
\texttt{e4497a6} & robertkodra & 2026-06-05 & $2{,}036{,}687{,}400$ & $-1{,}156{,}320$\\
\texttt{db60686} & robertkodra & 2026-06-05 & $2{,}037{,}843{,}720$ & $-2{,}595{,}120$\\
\texttt{bbf7b3a} & AnalyticETH & 2026-06-05 & $2{,}046{,}711{,}480$ & $-464{,}640$\\
\texttt{8c28287} & zuiris & 2026-06-05 & $2{,}047{,}176{,}120$ & $-1{,}277{,}760$\\
\texttt{8a9d274} & factory-sagar & 2026-06-05 & $2{,}048{,}453{,}880$ & $-781{,}440$\\
\texttt{2f24e2f} & robertkodra & 2026-06-05 & $2{,}049{,}235{,}320$ & $-1{,}156{,}320$\\
\texttt{6abbe60} & robertkodra & 2026-06-05 & $2{,}050{,}391{,}640$ & $-364{,}320$\\
\texttt{cf5e390} & robertkodra & 2026-06-05 & $2{,}050{,}755{,}960$ & $-1{,}140{,}480$\\
\texttt{c3cbcce} & newjordan & 2026-06-05 & $2{,}051{,}896{,}440$ & $-728{,}640$\\
\texttt{5ad23b1} & zuiris & 2026-06-05 & $2{,}052{,}625{,}080$ & $-1{,}029{,}210$\\
\texttt{ca7fd40} & mpjunior92 & 2026-06-05 & $2{,}055{,}555{,}480$ & $-4{,}812{,}720$\\
\texttt{229aeed} & 10d9e & 2026-06-05 & $2{,}060{,}368{,}200$ & $-498{,}960$\\
\texttt{a92d098} & newjordan & 2026-06-05 & $2{,}064{,}288{,}600$ & $-192{,}720$\\
\texttt{94e9418} & newjordan & 2026-06-05 & $2{,}064{,}481{,}320$ & $-1{,}869{,}120$\\
\texttt{ae3b97b} & 10d9e & 2026-06-05 & $2{,}091{,}370{,}926$ & $-530{,}688$\\
\texttt{05d68e5} & 10d9e & 2026-06-05 & $2{,}091{,}901{,}614$ & $-751{,}808$\\
\texttt{fa5347c} & factory-sagar & 2026-06-05 & $2{,}110{,}268{,}810$ & $-1{,}442{,}820$\\
\texttt{bc858e8} & 10d9e & 2026-06-05 & $2{,}111{,}711{,}630$ & $-720{,}020$\\
\texttt{fc27501} & alexander-sei & 2026-06-05 & $2{,}112{,}431{,}650$ & $-13{,}577{,}520$\\
\texttt{f0e2891} & robertkodra & 2026-06-05 & $2{,}126{,}009{,}170$ & $-1{,}237{,}100$\\
\texttt{b84d15c} & robertkodra & 2026-06-05 & $2{,}127{,}246{,}270$ & $-1{,}334{,}400$\\
\texttt{af0f90a} & 10d9e & 2026-06-05 & $2{,}128{,}580{,}670$ & $-720{,}020$\\
\texttt{dda7bfd} & robertkodra & 2026-06-05 & $2{,}129{,}300{,}690$ & $-811{,}760$\\
\texttt{98416e4} & robertkodra & 2026-06-05 & $2{,}130{,}112{,}450$ & $-261{,}320$\\
\texttt{4527ae1} & PhantasticUniverse & 2026-06-05 & $2{,}130{,}373{,}770$ & $-1{,}073{,}080$\\
\texttt{1991d1c} & newjordan & 2026-06-05 & $2{,}132{,}814{,}610$ & $-17{,}525{,}120$\\
\texttt{7c82c3c} & newjordan & 2026-06-05 & $2{,}150{,}339{,}730$ & $-4{,}692{,}640$\\
\texttt{247db26} & johnbxx & 2026-06-05 & $2{,}156{,}477{,}970$ & $-39{,}476{,}000$\\
\texttt{5b3887b} & newjordan & 2026-06-05 & $2{,}195{,}953{,}970$ & $-25{,}242{,}400$\\
\texttt{c6cc74e} & robertkodra & 2026-06-05 & $2{,}222{,}564{,}130$ & $-5{,}604{,}480$\\
\texttt{01260e8} & newjordan & 2026-06-05 & $2{,}228{,}168{,}610$ & $-29{,}556{,}960$\\
\texttt{9d30eb7} & johnbxx & 2026-06-05 & $2{,}257{,}725{,}570$ & $-8{,}651{,}360$\\
\texttt{d3e35ae} & mpjunior92 & 2026-06-03 & $2{,}405{,}410{,}905$ & $-1{,}701{,}880$\\
\texttt{cbe70bc} & mpjunior92 & 2026-06-03 & $2{,}407{,}112{,}785$ & $-2{,}829{,}240$\\
\texttt{353ac6d} & mpjunior92 & 2026-06-03 & $2{,}409{,}942{,}025$ & $-693{,}760$\\
\texttt{da42ce2} & harrigan & 2026-06-03 & $2{,}410{,}635{,}785$ & $-2{,}905{,}120$\\
\texttt{5b5a5d4} & teddyjfpender & 2026-06-03 & $2{,}430{,}923{,}007$ & $-3{,}025{,}184$\\
\texttt{b27f99c} & aburan28 & 2026-06-03 & $2{,}455{,}281{,}894$ & $-6{,}619{,}344$\\
\texttt{bdfc7df} & aburan28 & 2026-06-03 & $2{,}471{,}488{,}962$ & $-5{,}019{,}000$\\
\texttt{e75ea5c} & 10d9e & 2026-06-03 & $2{,}476{,}507{,}962$ & $-1{,}542{,}984$\\
\texttt{2bd707e} & aburan28 & 2026-06-03 & $2{,}478{,}050{,}946$ & $-1{,}497{,}096$\\
\texttt{b343178} & BitWonka & 2026-06-03 & $2{,}479{,}548{,}042$ & $-648{,}168$\\
\texttt{5d2f6cf} & BitWonka & 2026-06-03 & $2{,}480{,}196{,}210$ & $-1{,}132{,}860$\\
\texttt{238d366} & BitWonka & 2026-06-03 & $2{,}481{,}329{,}070$ & $-1{,}525{,}776$\\
\texttt{34a514a} & twangodev & 2026-06-03 & $2{,}484{,}807{,}954$ & $-1{,}135{,}728$\\
\texttt{5a2d910} & twangodev & 2026-06-03 & $2{,}485{,}943{,}682$ & $-7{,}995{,}984$\\
\texttt{113f346} & twangodev & 2026-06-03 & $2{,}498{,}876{,}289$ & $-6{,}632{,}028$\\
\texttt{144e07f} & phileigenlabs & 2026-06-03 & $2{,}505{,}508{,}317$ & $-473{,}304$\\
\texttt{d2b4bcf} & Epistetechnician & 2026-06-02 & $2{,}510{,}523{,}510$ & $-1{,}469{,}136$\\
\texttt{14b84f1} & 10d9e & 2026-06-02 & $2{,}533{,}577{,}850$ & $-1{,}489{,}456$\\
\texttt{47f30d4} & josusanmartin & 2026-06-02 & $2{,}592{,}421{,}194$ & $-1{,}467{,}984$\\
\texttt{1207861} & pldallairedemers & 2026-06-02 & $2{,}637{,}203{,}021$ & $-1{,}491{,}784$\\
\texttt{ecbf87b} & mpjunior92 & 2026-06-02 & $2{,}638{,}694{,}805$ & $-2{,}507{,}200$\\
\texttt{006e38b} & solimander & 2026-06-02 & $2{,}641{,}202{,}005$ & $-1{,}250{,}466$\\
\texttt{7408de1} & prasiddhnaik & 2026-06-02 & $2{,}736{,}895{,}656$ & $-58{,}127$\\
\texttt{6e7ca2c} & mpjunior92 & 2026-06-02 & $2{,}736{,}953{,}783$ & $-1{,}822{,}360$\\
\texttt{14fc786} & mpjunior92 & 2026-06-02 & $2{,}738{,}776{,}143$ & $-2{,}934{,}628$\\
\texttt{bb27ddd} & anupsv & 2026-06-02 & $2{,}769{,}217{,}908$ & $-14{,}632{,}176$\\
\texttt{4b68e94} & mpjunior92 & 2026-06-02 & $2{,}822{,}498{,}802$ & $-1{,}215{,}768$\\
\texttt{412312f} & mpjunior92 & 2026-06-02 & $2{,}823{,}714{,}570$ & $-6{,}656{,}160$\\
\texttt{8316db1} & mpjunior92 & 2026-06-02 & $2{,}830{,}370{,}730$ & $-1{,}215{,}768$\\
\texttt{1fd942d} & Gajesh2007 & 2026-06-02 & $2{,}831{,}586{,}498$ & $-1{,}086{,}720$\\
\texttt{eda50f2} & Epistetechnician & 2026-06-02 & $2{,}832{,}673{,}218$ & $-869{,}376$\\
\texttt{b694e22} & Gajesh2007 & 2026-06-02 & $2{,}833{,}542{,}594$ & $-2{,}859{,}432$\\
\texttt{dd103cd} & M3kko & 2026-06-02 & $2{,}873{,}320{,}661$ & $-9{,}151{,}501$\\
\texttt{ad02935} & Gajesh2007 & 2026-06-02 & $2{,}882{,}472{,}162$ & $-9{,}659{,}922$\\
\texttt{27530d2} & pldallairedemers & 2026-06-02 & $2{,}892{,}132{,}084$ & $-1{,}405{,}944$\\
\texttt{1846bf7} & megabyte0x & 2026-06-02 & $3{,}270{,}229{,}140$ & $-4{,}265{,}376$\\
\texttt{3c30191} & jtrose24 & 2026-06-02 & $3{,}315{,}144{,}636$ & $-49{,}839{,}696$\\
\texttt{6447611} & owizdom & 2026-06-02 & $3{,}538{,}424{,}844$ & $-236{,}823{,}456$\\
\texttt{8cb350c} & Gajesh2007 & 2026-06-02 & $4{,}068{,}676{,}284$ & $-27{,}833{,}616$\\
\texttt{564c4c3} & owizdom & 2026-06-02 & $4{,}096{,}509{,}900$ & $-34{,}503{,}360$\\
\texttt{00e3a20} & anupsv & 2026-06-02 & $4{,}131{,}013{,}260$ & $-17{,}007{,}168$\\
\texttt{541bd85} & josusanmartin & 2026-06-02 & $4{,}148{,}020{,}428$ & $-8{,}422{,}080$\\
\texttt{700d5a7} & 0xpg & 2026-06-02 & $5{,}148{,}949{,}806$ & $-8{,}808{,}800$\\
\texttt{6e71096} & Gajesh2007 & 2026-06-02 & $5{,}561{,}829{,}149$ & $-849{,}712$\\
\texttt{85ee8e7} & mpjunior92 & 2026-06-01 & $5{,}574{,}826{,}510$ & $-10{,}256{,}578$\\
\texttt{5136c0a} & mpjunior92 & 2026-06-01 & $5{,}597{,}330{,}024$ & $-25{,}066{,}504$\\
\texttt{49b7969} & anupsv & 2026-06-01 & $5{,}622{,}396{,}528$ & $-10{,}071{,}858$\\
\texttt{141b79a} & Gajesh2007 & 2026-06-01 & $5{,}935{,}088{,}235$ & $-40{,}093{,}476$\\
\texttt{9fa5a56} & anupsv & 2026-06-01 & $5{,}976{,}793{,}393$ & $-51{,}347{,}542$\\
\texttt{c7e1ae5} & saucegodbased & 2026-06-01 & $6{,}028{,}140{,}935$ & $-7{,}157{,}900$\\
\texttt{a25248f} & Gajesh2007 & 2026-06-01 & $6{,}035{,}298{,}835$ & $-4{,}811{,}956$\\
\texttt{404d630} & Gajesh2007 & 2026-06-01 & $6{,}040{,}110{,}791$ & $-413{,}504{,}956$\\
\texttt{0c25aca} & Gajesh2007 & 2026-06-01 & $6{,}453{,}615{,}747$ & $-8{,}280{,}074$\\
\texttt{bf19c9e} & Gajesh2007 & 2026-06-01 & $6{,}461{,}895{,}821$ & $-27{,}320{,}088$\\
\texttt{6eba4e3} & Gajesh2007 & 2026-06-01 & $6{,}489{,}215{,}909$ & $-3{,}204{,}892$\\
\texttt{e739b53} & anupsv & 2026-06-01 & $6{,}540{,}623{,}485$ & $-10{,}196{,}544$\\
\texttt{179ab10} & anupsv & 2026-06-01 & $6{,}550{,}820{,}029$ & $-13{,}535{,}358$\\
\texttt{fc8b9e6} & Gajesh2007 & 2026-06-01 & $6{,}616{,}811{,}249$ & $-10{,}113{,}420$\\
\texttt{13ac8da} & Gajesh2007 & 2026-06-01 & $6{,}764{,}917{,}436$ & $-100{,}441{,}500$\\
\texttt{b86e789} & Gajesh2007 & 2026-06-01 & $6{,}865{,}358{,}936$ & $-96{,}285{,}300$\\
\texttt{6da9882} & Gajesh2007 & 2026-06-01 & $6{,}964{,}659{,}240$ & $-110{,}103{,}840$\\
\texttt{36e8578} & Gajesh2007 & 2026-06-01 & $7{,}077{,}100{,}800$ & $-677{,}010{,}180$\\
\multicolumn{5}{@{}l}{\quad\itshape iteration/threshold tuning \small(37)}\\
\texttt{f861f87} & jackylee0424 & 2026-06-20 & $1{,}597{,}837{,}965$ & $-1{,}159$\\
\texttt{5f3a0e3} & bket7 & 2026-06-20 & $1{,}598{,}512{,}503$ & $-207{,}461$\\
\texttt{f0c1c42} & bket7 & 2026-06-20 & $1{,}598{,}719{,}964$ & $-1{,}335{,}168$\\
\texttt{0fa5c6f} & jieyilong & 2026-06-13 & $1{,}683{,}610{,}600$ & $-1{,}371{,}863$\\
\texttt{f6f9536} & BitWonka & 2026-06-10 & $1{,}768{,}166{,}425$ & $-6{,}559{,}925$\\
\texttt{1a7895c} & welttowelt & 2026-06-07 & $1{,}907{,}351{,}618$ & $-4{,}352{,}898$\\
\texttt{2c3b795} & zuiris & 2026-06-06 & $1{,}940{,}606{,}153$ & $-3{,}778{,}537$\\
\texttt{f5f0f61} & jieyilong & 2026-06-06 & $1{,}949{,}378{,}508$ & $-3{,}776{,}465$\\
\texttt{a6a92a4} & jieyilong & 2026-06-06 & $1{,}953{,}154{,}973$ & $-3{,}724{,}105$\\
\texttt{f37a0bc} & jackylee0424 & 2026-06-06 & $1{,}956{,}879{,}078$ & $-3{,}734{,}577$\\
\texttt{76fdaf2} & newjordan & 2026-06-06 & $1{,}986{,}336{,}599$ & $-3{,}872{,}037$\\
\texttt{c64c03f} & PhantasticUniverse & 2026-06-05 & $2{,}060{,}867{,}160$ & $-3{,}421{,}440$\\
\texttt{fec6d25} & 10d9e & 2026-06-05 & $2{,}092{,}653{,}422$ & $-17{,}615{,}388$\\
\texttt{8ef64e9} & stevenhao & 2026-06-04 & $2{,}381{,}382{,}450$ & $-18{,}066{,}455$\\
\texttt{39134ec} & stevenhao & 2026-06-04 & $2{,}399{,}448{,}905$ & $-2{,}981{,}000$\\
\texttt{c3c3f8d} & PhantasticUniverse & 2026-06-04 & $2{,}402{,}429{,}905$ & $-2{,}981{,}000$\\
\texttt{a392fd4} & aburan28 & 2026-06-03 & $2{,}439{,}135{,}048$ & $-3{,}078{,}384$\\
\texttt{311d6c3} & aburan28 & 2026-06-03 & $2{,}445{,}362{,}892$ & $-3{,}038{,}784$\\
\texttt{339fe8d} & aburan28 & 2026-06-03 & $2{,}482{,}854{,}846$ & $-1{,}953{,}108$\\
\texttt{f42ce5c} & Sam-Scolari & 2026-06-03 & $2{,}497{,}479{,}574$ & $-1{,}396{,}715$\\
\texttt{fd8e712} & pldallairedemers & 2026-06-02 & $2{,}535{,}067{,}306$ & $-4{,}459{,}572$\\
\texttt{7c29f79} & mmurrs & 2026-06-02 & $2{,}574{,}991{,}500$ & $-3{,}084{,}000$\\
\texttt{801b73e} & 0xpg & 2026-06-02 & $5{,}157{,}758{,}606$ & $-904{,}904$\\
\texttt{13a7a53} & antojoseph & 2026-06-02 & $5{,}182{,}912{,}575$ & $-421{,}200$\\
\texttt{17ae622} & Epistetechnician & 2026-06-02 & $5{,}183{,}333{,}775$ & $-1{,}684{,}800$\\
\texttt{0e726ac} & mpjunior92 & 2026-06-02 & $5{,}547{,}081{,}566$ & $-1{,}339{,}220$\\
\texttt{8eb6b5e} & jtrose24 & 2026-06-02 & $5{,}562{,}678{,}861$ & $-12{,}147{,}649$\\
\texttt{297f5e5} & jtrose24 & 2026-06-01 & $5{,}653{,}140{,}863$ & $-33{,}727{,}563$\\
\texttt{330186c} & anupsv & 2026-06-01 & $5{,}975{,}181{,}711$ & $-1{,}611{,}682$\\
\texttt{ac52c2e} & Gajesh2007 & 2026-06-01 & $6{,}496{,}336{,}865$ & $-11{,}720{,}484$\\
\texttt{f910ba3} & Gajesh2007 & 2026-06-01 & $7{,}756{,}453{,}320$ & $-1{,}173{,}480$\\
\texttt{a428a8c} & Gajesh2007 & 2026-06-01 & $7{,}757{,}626{,}800$ & $-8{,}036{,}490$\\
\texttt{77b87f1} & bxue-l2 & 2026-06-01 & $8{,}372{,}879{,}130$ & $-25{,}902{,}869$\\
\texttt{a3ee589} & philuponcrypto & 2026-05-31 & $8{,}405{,}420{,}100$ & $-40{,}029{,}990$\\
\texttt{1c400f2} & chainyoda & 2026-05-31 & $10{,}318{,}536{,}120$ & $-3{,}910{,}352$\\
\texttt{a444668} & unknown & 2026-05-31 & $10{,}397{,}877{,}812$ & $-690{,}540$\\
\texttt{9bd0748} & unknown & 2026-05-31 & $10{,}398{,}568{,}352$ & $-173{,}734{,}448$\\
\multicolumn{5}{@{}l}{\quad\itshape fold/carry truncation \small(37)}\\
\texttt{f6ce76d} & BitWonka & 2026-06-20 & $1{,}597{,}839{,}124$ & $-229{,}482$\\
\texttt{3df690f} & gopikannappan & 2026-06-20 & $1{,}607{,}030{,}040$ & $-1{,}870{,}580$\\
\texttt{31421df} & jieyilong & 2026-06-20 & $1{,}616{,}813{,}772$ & $-1{,}877{,}220$\\
\texttt{f265bb1} & jackylee0424 & 2026-06-19 & $1{,}646{,}703{,}035$ & $-9{,}320$\\
\texttt{550595a} & jackylee0424 & 2026-06-19 & $1{,}649{,}234{,}708$ & $-1{,}166$\\
\texttt{ed2715f} & gnuchev & 2026-06-19 & $1{,}649{,}235{,}874$ & $-461{,}736$\\
\texttt{764afda} & gnuchev & 2026-06-19 & $1{,}651{,}099{,}142$ & $-39{,}644$\\
\texttt{916c0e3} & DavetheSlayer & 2026-06-19 & $1{,}651{,}138{,}786$ & $-37{,}312$\\
\texttt{bc2334a} & BitWonka & 2026-06-19 & $1{,}651{,}176{,}098$ & $-5{,}923{,}280$\\
\texttt{fd89e69} & jieyilong & 2026-06-19 & $1{,}658{,}681{,}640$ & $-26{,}818$\\
\texttt{a9ac507} & jieyilong & 2026-06-19 & $1{,}658{,}708{,}458$ & $-26{,}818$\\
\texttt{c9c03de} & jackylee0424 & 2026-06-19 & $1{,}658{,}735{,}276$ & $-4{,}664$\\
\texttt{98e1322} & zuiris & 2026-06-11 & $1{,}709{,}962{,}980$ & $-3{,}134{,}180$\\
\texttt{c8f4536} & BitWonka & 2026-06-07 & $1{,}939{,}939{,}583$ & $-666{,}570$\\
\texttt{11ceae2} & welttowelt & 2026-06-06 & $1{,}960{,}613{,}655$ & $-7{,}278{,}040$\\
\texttt{004ffc0} & zuiris & 2026-06-06 & $1{,}970{,}059{,}399$ & $-1{,}350{,}888$\\
\texttt{69bd3d7} & Gajesh2007 & 2026-06-06 & $1{,}971{,}410{,}287$ & $-5{,}931{,}008$\\
\texttt{21fbfc7} & robertkodra & 2026-06-05 & $2{,}033{,}268{,}600$ & $-3{,}418{,}800$\\
\texttt{66c6dac} & mpjunior92 & 2026-06-05 & $2{,}054{,}166{,}840$ & $-1{,}388{,}640$\\
\texttt{438ef00} & mpjunior92 & 2026-06-05 & $2{,}089{,}123{,}794$ & $-2{,}247{,}132$\\
\texttt{5174a69} & PhantasticUniverse & 2026-06-05 & $2{,}131{,}446{,}850$ & $-1{,}367{,}760$\\
\texttt{657ae28} & PhantasticUniverse & 2026-06-05 & $2{,}221{,}196{,}370$ & $-1{,}367{,}760$\\
\texttt{cc5584e} & PhantasticUniverse & 2026-06-05 & $2{,}379{,}298{,}050$ & $-2{,}084{,}400$\\
\texttt{40574d3} & mpjunior92 & 2026-06-02 & $2{,}616{,}750{,}555$ & $-3{,}693{,}942$\\
\texttt{7787f81} & mpjunior92 & 2026-06-02 & $2{,}620{,}444{,}497$ & $-10{,}554{,}777$\\
\texttt{f8a36ba} & Gajesh2007 & 2026-06-02 & $2{,}893{,}538{,}028$ & $-227{,}470{,}872$\\
\texttt{115ab0e} & xadenryan & 2026-06-02 & $5{,}166{,}788{,}002$ & $-32{,}096$\\
\texttt{61bdeb0} & antojoseph & 2026-06-02 & $5{,}180{,}304{,}536$ & $-48{,}576$\\
\texttt{8d83e8e} & 0xpg & 2026-06-02 & $5{,}182{,}432{,}650$ & $-479{,}925$\\
\texttt{3ab1c72} & anupsv & 2026-06-02 & $5{,}548{,}420{,}786$ & $-1{,}108{,}320$\\
\texttt{3f534f2} & Gajesh2007 & 2026-06-02 & $5{,}549{,}529{,}106$ & $-12{,}300{,}043$\\
\texttt{1b913c5} & anupsv & 2026-06-01 & $5{,}585{,}083{,}088$ & $-12{,}246{,}936$\\
\texttt{ba05d3a} & Gajesh2007 & 2026-06-01 & $5{,}686{,}868{,}426$ & $-195{,}285{,}984$\\
\texttt{d6551e8} & solimander & 2026-06-01 & $5{,}882{,}154{,}410$ & $-52{,}933{,}825$\\
\texttt{a97b4e9} & Gajesh2007 & 2026-06-01 & $6{,}508{,}057{,}349$ & $-18{,}430{,}438$\\
\texttt{2abe7f4} & Gajesh2007 & 2026-06-01 & $6{,}564{,}355{,}387$ & $-52{,}455{,}862$\\
\texttt{1e18b4d} & Gajesh2007 & 2026-06-01 & $6{,}626{,}924{,}669$ & $-137{,}992{,}767$\\
\multicolumn{5}{@{}l}{\quad\itshape dead-gate/self-inverse removal \small(21)}\\
\texttt{9eea46c} & jackylee0424 & 2026-07-18 & $1{,}519{,}161{,}984$ & $-8{,}064$\\
\texttt{a505e6d} & mochimodev & 2026-07-11 & $1{,}519{,}170{,}048$ & $-2{,}348{,}928$\\
\texttt{6dafa07} & BitWonka & 2026-06-26 & $1{,}576{,}955{,}794$ & $-894{,}728$\\
\texttt{da51a48} & jieyilong & 2026-06-23 & $1{,}577{,}865{,}511$ & $-97{,}609$\\
\texttt{985eaec} & BitWonka & 2026-06-23 & $1{,}577{,}963{,}120$ & $-1{,}086{,}640$\\
\texttt{27d4627} & BitWonka & 2026-06-22 & $1{,}579{,}049{,}760$ & $-321{,}368$\\
\texttt{6c0769f} & BitWonka & 2026-06-22 & $1{,}579{,}371{,}128$ & $-1{,}945{,}292$\\
\texttt{20b9a1d} & mpjunior92 & 2026-06-21 & $1{,}581{,}316{,}420$ & $-1{,}439{,}478$\\
\texttt{4a90d04} & zuiris & 2026-06-21 & $1{,}582{,}755{,}898$ & $-13{,}950{,}606$\\
\texttt{9af02f7} & gnuchev & 2026-06-21 & $1{,}597{,}055{,}640$ & $-282{,}796$\\
\texttt{9d524b7} & BitWonka & 2026-06-20 & $1{,}597{,}538{,}943$ & $-150{,}787$\\
\texttt{6ba606a} & jieyilong & 2026-06-20 & $1{,}597{,}689{,}730$ & $-148{,}235$\\
\texttt{a47dc6e} & PhantasticUniverse & 2026-06-19 & $1{,}644{,}083{,}652$ & $-1{,}186{,}116$\\
\texttt{ba3efc1} & BitWonka & 2026-06-18 & $1{,}672{,}133{,}328$ & $-830{,}448$\\
\texttt{7822c37} & BitWonka & 2026-06-09 & $1{,}774{,}746{,}910$ & $-1{,}322{,}265$\\
\texttt{b8ce940} & BitWonka & 2026-06-09 & $1{,}776{,}069{,}175$ & $-651{,}495$\\
\texttt{b55ede3} & welttowelt & 2026-06-06 & $1{,}968{,}567{,}139$ & $-226{,}336$\\
\texttt{975b73f} & josusanmartin & 2026-06-02 & $2{,}590{,}854{,}522$ & $-1{,}515{,}843$\\
\texttt{908521d} & anupsv & 2026-06-02 & $5{,}121{,}484{,}498$ & $-27{,}465{,}308$\\
\texttt{c8e508f} & Gajesh2007 & 2026-06-01 & $8{,}367{,}457{,}560$ & $-5{,}421{,}570$\\
\texttt{a16788e} & unknown & 2026-05-30 & $10{,}579{,}872{,}520$ & $-118{,}867{,}397$\\
\addlinespace[2pt]
\multicolumn{5}{@{}l}{\rule{0pt}{2.6ex}\textbf{Register and Scratch Allocation}~\small(50)}\\[1pt]
\multicolumn{5}{@{}l}{\quad\itshape ancilla-lifetime / venting \small(30)}\\
\texttt{d11bdbb} & BitWonka & 2026-06-20 & $1{,}600{,}244{,}049$ & $-6{,}765{,}039$\\
\texttt{fed64cf} & nasqret & 2026-06-20 & $1{,}608{,}900{,}620$ & $-5{,}159{,}212$\\
\texttt{b310de9} & BitWonka & 2026-06-19 & $1{,}642{,}623{,}526$ & $-924{,}686$\\
\texttt{f8d23a9} & BitWonka & 2026-06-19 & $1{,}645{,}269{,}768$ & $-1{,}030{,}177$\\
\texttt{cea9f5f} & BitWonka & 2026-06-19 & $1{,}646{,}712{,}355$ & $-2{,}059{,}451$\\
\texttt{cf3c6f1} & BitWonka & 2026-06-12 & $1{,}701{,}341{,}166$ & $-712{,}854$\\
\texttt{9191f81} & zuiris & 2026-06-11 & $1{,}708{,}341{,}222$ & $-1{,}621{,}758$\\
\texttt{572bba4} & zuiris & 2026-06-10 & $1{,}743{,}798{,}012$ & $-3{,}488{,}606$\\
\texttt{da398df} & BitWonka & 2026-06-08 & $1{,}786{,}833{,}620$ & $-11{,}871{,}920$\\
\texttt{89abe1b} & zuiris & 2026-06-06 & $1{,}946{,}400{,}084$ & $-2{,}978{,}424$\\
\texttt{33c072d} & jieyilong & 2026-06-06 & $1{,}968{,}793{,}475$ & $-449{,}108$\\
\texttt{a5e8bdf} & runeape-sats & 2026-06-06 & $1{,}977{,}341{,}295$ & $-288{,}051$\\
\texttt{571e67c} & runeape-sats & 2026-06-06 & $1{,}978{,}456{,}675$ & $-329{,}827$\\
\texttt{06b07ee} & teddyjfpender & 2026-06-05 & $2{,}066{,}350{,}440$ & $-22{,}773{,}354$\\
\texttt{1eae277} & newjordan & 2026-06-05 & $2{,}155{,}032{,}370$ & $-1{,}445{,}600$\\
\texttt{250774e} & 10d9e & 2026-06-02 & $2{,}578{,}075{,}500$ & $-12{,}779{,}022$\\
\texttt{46c3e3a} & bxue-l2 & 2026-06-02 & $2{,}593{,}889{,}178$ & $-1{,}682{,}159$\\
\texttt{7021abe} & anupsv & 2026-06-02 & $2{,}614{,}737{,}018$ & $-544{,}601$\\
\texttt{287595e} & 10d9e & 2026-06-02 & $2{,}615{,}519{,}241$ & $-1{,}231{,}314$\\
\texttt{550895c} & solimander & 2026-06-02 & $2{,}647{,}454{,}335$ & $-84{,}484{,}816$\\
\texttt{36dcf6b} & pldallairedemers & 2026-06-02 & $2{,}744{,}218{,}087$ & $-1{,}746{,}797$\\
\texttt{68e3653} & saucegodbased & 2026-06-02 & $2{,}783{,}850{,}084$ & $-38{,}648{,}718$\\
\texttt{0435f04} & nandy-technologies & 2026-06-02 & $5{,}160{,}257{,}102$ & $-5{,}760{,}596$\\
\texttt{ccd7530} & Gajesh2007 & 2026-06-02 & $5{,}166{,}820{,}098$ & $-13{,}484{,}438$\\
\texttt{9899c06} & antojoseph & 2026-06-02 & $5{,}180{,}353{,}112$ & $-2{,}079{,}538$\\
\texttt{233a44c} & Gajesh2007 & 2026-06-02 & $5{,}185{,}018{,}575$ & $-362{,}062{,}991$\\
\texttt{0e32587} & Gajesh2007 & 2026-06-01 & $6{,}961{,}644{,}236$ & $-3{,}015{,}004$\\
\texttt{74a1a8b} & cryptogakusei & 2026-05-31 & $9{,}603{,}905{,}752$ & $-433{,}280$\\
\texttt{b827c9e} & unknown & 2026-05-31 & $10{,}395{,}860{,}352$ & $-2{,}017{,}460$\\
\texttt{bc9728a} & unknown & 2026-05-30 & $10{,}572{,}584{,}432$ & $-7{,}288{,}088$\\
\multicolumn{5}{@{}l}{\quad\itshape scratch/ancilla reuse \small(17)}\\
\texttt{461a4a3} & BitWonka & 2026-06-11 & $1{,}703{,}067{,}769$ & $-1{,}716{,}956$\\
\texttt{420e0c2} & BitWonka & 2026-06-11 & $1{,}705{,}055{,}670$ & $-2{,}814{,}186$\\
\texttt{997dbd6} & BitWonka & 2026-06-11 & $1{,}713{,}124{,}000$ & $-3{,}050{,}108$\\
\texttt{8983da8} & SamrendraS & 2026-06-08 & $1{,}822{,}107{,}738$ & $-1{,}067{,}340$\\
\texttt{ea8ce7b} & jieyilong & 2026-06-07 & $1{,}916{,}455{,}744$ & $-1{,}488{,}336$\\
\texttt{3409fbd} & zuiris & 2026-06-07 & $1{,}920{,}798{,}194$ & $-1{,}491{,}661$\\
\texttt{13a01b8} & nikhiljha & 2026-06-03 & $2{,}413{,}540{,}905$ & $-17{,}382{,}102$\\
\texttt{e0cfe2b} & nikhiljha & 2026-06-03 & $2{,}433{,}948{,}191$ & $-3{,}091{,}060$\\
\texttt{24a4076} & nikhiljha & 2026-06-03 & $2{,}437{,}039{,}251$ & $-2{,}095{,}797$\\
\texttt{3166bbd} & nikhiljha & 2026-06-03 & $2{,}442{,}213{,}432$ & $-3{,}149{,}460$\\
\texttt{dd188f8} & nikhiljha & 2026-06-03 & $2{,}448{,}401{,}676$ & $-6{,}880{,}218$\\
\texttt{1d2cbc9} & mpjunior92 & 2026-06-02 & $2{,}505{,}981{,}621$ & $-2{,}913{,}693$\\
\texttt{6189d5f} & alexander-sei & 2026-06-02 & $2{,}508{,}895{,}314$ & $-1{,}628{,}196$\\
\texttt{8ab5f90} & pldallairedemers & 2026-06-02 & $2{,}511{,}992{,}646$ & $-21{,}585{,}204$\\
\texttt{92a247e} & mpjunior92 & 2026-06-02 & $2{,}539{,}526{,}878$ & $-35{,}464{,}622$\\
\texttt{a8688f8} & josusanmartin & 2026-06-02 & $5{,}166{,}017{,}698$ & $-770{,}304$\\
\texttt{666b591} & Gajesh2007 & 2026-05-31 & $10{,}347{,}216{,}548$ & $-48{,}643{,}804$\\
\multicolumn{5}{@{}l}{\quad\itshape in-place mutation \small(3)}\\
\texttt{fe29b53} & josusanmartin & 2026-06-02 & $2{,}615{,}281{,}619$ & $-237{,}622$\\
\texttt{b113c6f} & mpjunior92 & 2026-06-02 & $2{,}630{,}999{,}274$ & $-6{,}203{,}747$\\
\texttt{d19dbb5} & Gajesh2007 & 2026-05-31 & $8{,}445{,}450{,}090$ & $-1{,}145{,}844{,}506$\\
\addlinespace[2pt]
\multicolumn{5}{@{}l}{\rule{0pt}{2.6ex}\textbf{Uncompute Strategy}~\small(22)}\\[1pt]
\multicolumn{5}{@{}l}{\quad\itshape measurement uncompute \small(22)}\\
\texttt{d44cad3} & BitWonka & 2026-06-26 & $1{,}571{,}592{,}960$ & $-5{,}362{,}834$\\
\texttt{5c34dd1} & BitWonka & 2026-06-20 & $1{,}598{,}068{,}606$ & $-443{,}897$\\
\texttt{d636d62} & nasqret & 2026-06-11 & $1{,}707{,}869{,}856$ & $-471{,}366$\\
\texttt{08c5068} & BitWonka & 2026-06-10 & $1{,}747{,}286{,}618$ & $-12{,}457{,}386$\\
\texttt{b7515d5} & zuiris & 2026-06-09 & $1{,}780{,}286{,}545$ & $-3{,}442{,}515$\\
\texttt{c27e8a5} & zuiris & 2026-06-09 & $1{,}783{,}729{,}060$ & $-1{,}818{,}275$\\
\texttt{98dd2ad} & BitWonka & 2026-06-08 & $1{,}798{,}705{,}540$ & $-21{,}936{,}161$\\
\texttt{bfd3fa6} & BitWonka & 2026-06-08 & $1{,}825{,}275{,}400$ & $-66{,}073{,}800$\\
\texttt{e321f72} & BitWonka & 2026-06-07 & $1{,}892{,}934{,}834$ & $-888{,}795$\\
\texttt{bde4caa} & zuiris & 2026-06-07 & $1{,}896{,}965{,}826$ & $-2{,}596{,}188$\\
\texttt{a88c9a1} & welttowelt & 2026-06-07 & $1{,}906{,}003{,}826$ & $-1{,}347{,}792$\\
\texttt{94535d1} & welttowelt & 2026-06-07 & $1{,}917{,}944{,}080$ & $-2{,}854{,}114$\\
\texttt{fb83e6c} & nikhiljha & 2026-06-03 & $2{,}461{,}901{,}238$ & $-9{,}587{,}724$\\
\texttt{985ae0f} & josusanmartin & 2026-06-02 & $2{,}841{,}822{,}042$ & $-26{,}135{,}195$\\
\texttt{0aa33ed} & Gajesh2007 & 2026-06-02 & $2{,}871{,}482{,}706$ & $-1{,}837{,}955$\\
\texttt{acf2bdb} & saucegodbased & 2026-06-02 & $3{,}121{,}008{,}900$ & $-40{,}650{,}120$\\
\texttt{4b9cfbb} & saucegodbased & 2026-06-02 & $3{,}274{,}494{,}516$ & $-40{,}650{,}120$\\
\texttt{c813ee5} & saucegodbased & 2026-06-02 & $3{,}364{,}984{,}332$ & $-173{,}440{,}512$\\
\texttt{7e660f9} & saucegodbased & 2026-06-02 & $3{,}775{,}248{,}300$ & $-293{,}427{,}984$\\
\texttt{ce60f0e} & Gajesh2007 & 2026-06-01 & $7{,}754{,}110{,}980$ & $-2{,}342{,}340$\\
\texttt{81ff75b} & Gajesh2007 & 2026-05-31 & $10{,}322{,}446{,}472$ & $-21{,}997{,}084$\\
\texttt{e33b400} & cryptogakusei & 2026-05-31 & $10{,}344{,}443{,}556$ & $-2{,}772{,}992$\\
\addlinespace[2pt]
\multicolumn{5}{@{}l}{\rule{0pt}{2.6ex}\textbf{Constant Propagation and Classical Specialization}~\small(19)}\\[1pt]
\multicolumn{5}{@{}l}{\quad\itshape host-derived / classical specialization \small(19)}\\
\texttt{cde752d} & BitWonka & 2026-06-21 & $1{,}596{,}706{,}504$ & $-349{,}136$\\
\texttt{f8e215b} & gopikannappan & 2026-06-20 & $1{,}597{,}382{,}478$ & $-156{,}465$\\
\texttt{662e267} & bket7 & 2026-06-20 & $1{,}600{,}055{,}132$ & $-188{,}917$\\
\texttt{7b7bd12} & BitWonka & 2026-06-20 & $1{,}614{,}062{,}156$ & $-70{,}882$\\
\texttt{d2643bc} & nasqret & 2026-06-19 & $1{,}618{,}690{,}992$ & $-377{,}136$\\
\texttt{fa7126d} & gopikannappan & 2026-06-19 & $1{,}643{,}656{,}464$ & $-427{,}188$\\
\texttt{9798bc9} & gopikannappan & 2026-06-19 & $1{,}646{,}299{,}945$ & $-356{,}490$\\
\texttt{b02b354} & gopikannappan & 2026-06-19 & $1{,}648{,}771{,}806$ & $-462{,}902$\\
\texttt{497cc20} & gopikannappan & 2026-06-19 & $1{,}649{,}697{,}610$ & $-1{,}378{,}212$\\
\texttt{c69b6c1} & zuiris & 2026-06-05 & $2{,}023{,}711{,}363$ & $-1{,}534{,}277$\\
\texttt{8117d98} & mpjunior92 & 2026-06-02 & $2{,}642{,}452{,}471$ & $-5{,}001{,}864$\\
\texttt{17aad9a} & mpjunior92 & 2026-06-02 & $2{,}731{,}939{,}151$ & $-4{,}956{,}505$\\
\texttt{335ac78} & solimander & 2026-06-02 & $2{,}741{,}710{,}771$ & $-2{,}507{,}316$\\
\texttt{075c0c6} & ptrdsh & 2026-06-02 & $2{,}745{,}964{,}884$ & $-5{,}017{,}824$\\
\texttt{9805d0c} & Epistetechnician & 2026-06-02 & $2{,}836{,}402{,}026$ & $-5{,}420{,}016$\\
\texttt{0261289} & Epistetechnician & 2026-06-02 & $2{,}867{,}957{,}237$ & $-3{,}525{,}469$\\
\texttt{b60eec2} & saucegodbased & 2026-06-01 & $8{,}398{,}781{,}999$ & $-6{,}638{,}101$\\
\texttt{3bbccd3} & mmurrs & 2026-05-31 & $9{,}591{,}294{,}596$ & $-16{,}248$\\
\texttt{8631b04} & unknown & 2026-05-30 & $10{,}572{,}302{,}800$ & $-281{,}632$\\
\addlinespace[2pt]
\multicolumn{5}{@{}l}{\rule{0pt}{2.6ex}\textbf{Strength Reduction}~\small(14)}\\[1pt]
\multicolumn{5}{@{}l}{\quad\itshape fast-adder reroute \small(9)}\\
\texttt{2a87f33} & Gajesh2007 & 2026-06-09 & $1{,}776{,}720{,}670$ & $-2{,}983{,}770$\\
\texttt{82f7a95} & newjordan & 2026-06-07 & $1{,}912{,}381{,}024$ & $-4{,}074{,}720$\\
\texttt{639f12c} & runeape-sats & 2026-06-06 & $1{,}985{,}678{,}387$ & $-658{,}212$\\
\texttt{df83d16} & bxue-l2 & 2026-06-02 & $2{,}595{,}571{,}337$ & $-19{,}165{,}681$\\
\texttt{53f0bdb} & anupsv & 2026-06-01 & $5{,}632{,}468{,}386$ & $-20{,}672{,}477$\\
\texttt{d4959a1} & Gajesh2007 & 2026-06-01 & $6{,}492{,}420{,}801$ & $-3{,}916{,}064$\\
\texttt{0be8d11} & Gajesh2007 & 2026-06-01 & $6{,}526{,}487{,}787$ & $-14{,}135{,}698$\\
\texttt{04b3a76} & mmurrs & 2026-05-31 & $9{,}591{,}310{,}844$ & $-12{,}594{,}908$\\
\texttt{168048c} & unknown & 2026-05-30 & $10{,}698{,}739{,}917$ & $-5{,}834{,}478$\\
\multicolumn{5}{@{}l}{\quad\itshape solinas / NAF fold \small(5)}\\
\texttt{aacf05c} & gnuchev & 2026-06-20 & $1{,}614{,}133{,}038$ & $-1{,}831{,}866$\\
\texttt{e25c7d8} & 0xLucqs & 2026-06-20 & $1{,}615{,}964{,}904$ & $-848{,}868$\\
\texttt{4ea8b74} & alexander-sei & 2026-06-19 & $1{,}641{,}531{,}000$ & $-1{,}092{,}526$\\
\texttt{ed94ad2} & SamrendraS & 2026-06-09 & $1{,}779{,}704{,}440$ & $-582{,}105$\\
\texttt{6bf73fe} & BitWonka & 2026-06-07 & $1{,}922{,}289{,}855$ & $-17{,}461{,}520$\\
\addlinespace[2pt]
\multicolumn{5}{@{}l}{\rule{0pt}{2.6ex}\textbf{Fusion}~\small(12)}\\[1pt]
\multicolumn{5}{@{}l}{\quad\itshape gate/op fusion \small(7)}\\
\texttt{12c7337} & PhantasticUniverse & 2026-06-19 & $1{,}643{,}554{,}032$ & $-102{,}432$\\
\texttt{b1dec1e} & nasqret & 2026-06-19 & $1{,}657{,}099{,}378$ & $-1{,}253{,}450$\\
\texttt{84d5b0e} & rubenmarcus & 2026-06-15 & $1{,}676{,}067{,}120$ & $-1{,}794{,}780$\\
\texttt{8a47cf5} & johnbxx & 2026-06-06 & $1{,}993{,}816{,}760$ & $-19{,}572{,}891$\\
\texttt{e4edca0} & nikhiljha & 2026-06-03 & $2{,}493{,}939{,}666$ & $-3{,}539{,}908$\\
\texttt{9b6b9d6} & Epistetechnician & 2026-06-02 & $3{,}161{,}659{,}020$ & $-108{,}570{,}120$\\
\texttt{f9fae31} & Gajesh2007 & 2026-06-01 & $7{,}074{,}763{,}080$ & $-2{,}337{,}720$\\
\multicolumn{5}{@{}l}{\quad\itshape boundary cswap-merge \small(5)}\\
\texttt{422f21d} & mochimodev & 2026-07-07 & $1{,}521{,}518{,}976$ & $-50{,}073{,}984$\\
\texttt{cef001a} & owizdom & 2026-06-02 & $5{,}120{,}690{,}122$ & $-794{,}376$\\
\texttt{cd34b79} & antojoseph & 2026-06-02 & $5{,}158{,}663{,}510$ & $-1{,}593{,}592$\\
\texttt{36a2989} & Gajesh2007 & 2026-06-01 & $7{,}765{,}663{,}290$ & $-601{,}794{,}270$\\
\texttt{9bcc27d} & Gajesh2007 & 2026-05-31 & $9{,}604{,}339{,}032$ & $-714{,}197{,}088$\\
\addlinespace[2pt]
\multicolumn{5}{@{}l}{\rule{0pt}{2.6ex}\textbf{Windowing}~\small(8)}\\[1pt]
\multicolumn{5}{@{}l}{\quad\itshape windowed carry/shift blocks \small(5)}\\
\texttt{7689eac} & welttowelt & 2026-06-10 & $1{,}759{,}744{,}004$ & $-5{,}745{,}766$\\
\texttt{2eab923} & PhantasticUniverse & 2026-06-05 & $2{,}040{,}438{,}840$ & $-6{,}272{,}640$\\
\texttt{a91b626} & robertkodra & 2026-06-05 & $2{,}053{,}654{,}290$ & $-512{,}550$\\
\texttt{a772a45} & robertkodra & 2026-06-05 & $2{,}266{,}376{,}930$ & $-5{,}077{,}764$\\
\texttt{7297f4f} & fortunexbt & 2026-06-02 & $2{,}592{,}370{,}365$ & $-50{,}829$\\
\multicolumn{5}{@{}l}{\quad\itshape K2 transcript pair-compressor \small(2)}\\
\texttt{9a81017} & anshu4321 & 2026-06-05 & $2{,}017{,}979{,}899$ & $-2{,}204{,}458$\\
\texttt{0780f67} & johnbxx & 2026-06-05 & $2{,}271{,}454{,}694$ & $-107{,}843{,}356$\\
\multicolumn{5}{@{}l}{\quad\itshape two-jump inversion base \small(1)}\\
\texttt{cddd5df} & pldallairedemers & 2026-06-02 & $4{,}156{,}442{,}508$ & $-964{,}247{,}614$\\
\addlinespace[2pt]
\multicolumn{5}{@{}l}{\rule{0pt}{2.6ex}\textbf{Codec / Encoding}~\small(7)}\\[1pt]
\multicolumn{5}{@{}l}{\quad\itshape trailmix / K5 codec \small(7)}\\
\texttt{ab1b2d6} & PhantasticUniverse & 2026-06-19 & $1{,}658{,}770{,}256$ & $-1{,}389{,}940$\\
\texttt{bdb1d22} & tob-joe & 2026-06-19 & $1{,}660{,}163{,}697$ & $-8{,}908{,}303$\\
\texttt{35ceb01} & BitWonka & 2026-06-15 & $1{,}674{,}533{,}568$ & $-1{,}533{,}552$\\
\texttt{674d0d8} & nasqret & 2026-06-14 & $1{,}678{,}948{,}830$ & $-2{,}076{,}765$\\
\texttt{cf310ec} & nasqret & 2026-06-13 & $1{,}681{,}025{,}595$ & $-2{,}058{,}141$\\
\texttt{bb579bb} & BitWonka & 2026-06-13 & $1{,}684{,}982{,}463$ & $-12{,}415{,}650$\\
\texttt{6953d1b} & BitWonka & 2026-06-12 & $1{,}697{,}398{,}113$ & $-2{,}254{,}919$\\
\addlinespace[2pt]
\multicolumn{5}{@{}l}{\rule{0pt}{2.6ex}\textbf{Algorithmic Substitution}~\small(2)}\\[1pt]
\multicolumn{5}{@{}l}{\quad\itshape multiplier/squarer swap \small(2)}\\
\texttt{28fe2f2} & alexander-sei & 2026-06-19 & $1{,}619{,}139{,}132$ & $-22{,}382{,}556$\\
\texttt{b6d6f41} & mpjunior92 & 2026-06-02 & $2{,}750{,}982{,}708$ & $-18{,}235{,}200$\\
\addlinespace[2pt]
\multicolumn{5}{@{}l}{\rule{0pt}{2.6ex}\textbf{Verifier Search}~\small(19)}\\[1pt]
\multicolumn{5}{@{}l}{\quad\itshape nonce/island reroll \small(19)}\\
\texttt{4cd1b2f} & welttowelt & 2026-06-25 & $1{,}577{,}850{,}522$ & $-3{,}459$\\
\texttt{9b09c7e} & welttowelt & 2026-06-25 & $1{,}577{,}853{,}981$ & $-3{,}459$\\
\texttt{d17af14} & welttowelt & 2026-06-25 & $1{,}577{,}857{,}440$ & $-8{,}071$\\
\texttt{c07bf74} & welttowelt & 2026-06-21 & $1{,}597{,}338{,}436$ & $-40{,}565$\\
\texttt{85ee6af} & newjordan & 2026-06-21 & $1{,}597{,}379{,}001$ & $-3{,}477$\\
\texttt{42b56c6} & welttowelt & 2026-06-20 & $1{,}607{,}009{,}088$ & $-20{,}952$\\
\texttt{94d44be} & welttowelt & 2026-06-20 & $1{,}614{,}059{,}832$ & $-2{,}324$\\
\texttt{883f71a} & nasqret & 2026-06-19 & $1{,}619{,}068{,}128$ & $-27{,}936$\\
\texttt{533ef88} & gopikannappan & 2026-06-19 & $1{,}619{,}096{,}064$ & $-12{,}804$\\
\texttt{41df0b5} & gopikannappan & 2026-06-19 & $1{,}619{,}108{,}868$ & $-17{,}460$\\
\texttt{3b05e0a} & jackylee0424 & 2026-06-19 & $1{,}619{,}126{,}328$ & $-12{,}804$\\
\texttt{eb089b1} & gopikannappan & 2026-06-19 & $1{,}641{,}521{,}688$ & $-9{,}312$\\
\texttt{6a9db88} & jackylee0424 & 2026-06-19 & $1{,}643{,}548{,}212$ & $-5{,}820$\\
\texttt{fdb103e} & jackylee0424 & 2026-06-19 & $1{,}646{,}656{,}435$ & $-46{,}600$\\
\texttt{01560c7} & gnuchev & 2026-06-19 & $1{,}651{,}075{,}822$ & $-23{,}320$\\
\texttt{70bf11a} & rubenmarcus & 2026-06-19 & $1{,}658{,}352{,}828$ & $-9{,}328$\\
\texttt{5407215} & jackylee0424 & 2026-06-19 & $1{,}658{,}739{,}940$ & $-30{,}316$\\
\texttt{615ce9a} & jackylee0424 & 2026-06-19 & $1{,}660{,}160{,}196$ & $-3{,}501$\\
\texttt{a4db9a5} & SamrendraS & 2026-06-08 & $1{,}820{,}670{,}235$ & $-1{,}437{,}503$\\
\addlinespace[2pt]
\multicolumn{5}{@{}l}{\rule{0pt}{2.6ex}\textbf{Neutral / Mechanical}~\small(3)}\\[1pt]
\multicolumn{5}{@{}l}{\quad\itshape DUMMY\_TOFFOLIS padding change \small(3)}\\
\texttt{f43a73e} & unknown & 2026-05-30 & $10{,}704{,}574{,}395$ & $-47{,}186{,}700$\\
\texttt{ed34c00} & unknown & 2026-05-30 & $10{,}751{,}761{,}095$ & $-1{,}683{,}300$\\
\texttt{6f7c159} & unknown & 2026-05-30 & $10{,}753{,}444{,}395$ & $0$\\
\addlinespace[2pt]
\multicolumn{5}{@{}l}{\rule{0pt}{2.6ex}\textbf{Unscored bootstrap (\texttt{DUMMY\_TOFFOLIS})}~\small(4)}\\[1pt]
\texttt{15a06af} & unknown & 2026-05-29 & \emph{(unscored)} & ---\\
\texttt{971d801} & unknown & 2026-05-30 & \emph{(unscored)} & ---\\
\texttt{c55911f} & unknown & 2026-05-29 & \emph{(unscored)} & ---\\
\texttt{ca1bf33} & unknown & 2026-05-30 & \emph{(unscored)} & ---\\
\end{longtable}
}
